# Supplementary material for: Prototype-based Incremental Few-Shot Semantic Segmentation
Source: arXiv:2012.01415 source file (2021-10-18)
Supplement: Supplementary file 1 [file supp_mat.tex]

\section{Implementation details}
\vspace{10pt}
\subsection{Training protocol} \label{sec:training-protocol}
In this section, we provide additional details on the training protocol used in our experiments. Note that we adopt the same protocol for all the methods, to ensure a fair comparison. 

When fine-tuning we follow \cite{chen2018encoder}, using SGD as optimizer with momentum $0.9$, weight decay $10^{-4}$ and a polynomial learning rate policy, \ie $\text{lr} = \text{lr}_{\text{init}} (1- \frac{\text{iter}}{\max\_\text{iter}})^{0.9}$. 
During training, we apply the same data augmentation of \cite{chen2018encoder}, performing random scaling and horizontal flipping, % of the training images, 
with a crop-size of $512\times512$. While the previous hyperparameters are shared across settings, we use a different learning rate and number of training iterations depending on the dataset, number of shots and learning steps. In particular, in the base step we train the network for 30 epochs on Pascal-VOC and 20 epochs on COCO using learning rate $10^{-2}$ and batch size 24. For the FSL step t, we set the batch size to $\min(10, |\set D_t|)$. In the FSL steps of VOC-SS, we train for 1000 iterations with learning rate $10^{-3}$, and for 200 iterations per step for VOC-MS, with learning rate $10^{-4}$.
On COCO FSL steps we use a learning rate $10^{-3}$, training the model for 2000 iterations on COCO-SS, and 100 iterations on every step of COCO-MS. These training hyperparameters are shared by all methods.

\subsection{Adapting baselines to iFSS and hyperparameters choice}
In this section, we describe how we adapt the baselines reported in the main paper to iFSS and the value of their hyperparameters. We set the hyperparameters specific of each approach in the VOC-SS and COCO-SS 1-shot settings, using the first split of each dataset (\ie 5-0 for VOC, and 20-0 for COCO) and maintaining the same values across all other shots, splits and number of learning steps.

For Weight Imprinting (WI), we adapted the work of \cite{qi2018low} from image classification. In particular, we %as described in Sec.~4.1 of the main paper.
replaced the image-level feature extractor of \cite{qi2018low} with masked average pooling (MAP), as described in Sec.~4.1 of the paper. This method does not require additional hyperparameters, and we initialize the prototypes for new classes while keeping the prototypes of old ones unaltered. 

%\fabio{Come adattato su segm.}
Similarly, for Dynamic Weight Imprinting \cite{gidaris2018dynamic} (DWI), we implemented the classifier using the same attention mechanism and weight generator of \cite{gidaris2018dynamic}, but we replaced the class-specific image-level features with the ones extracted through MAP. DWI uses a second meta-learning training stage on the base classes {to refine the weight generator}. %In both stage we compute the loss (i.e. cross-entropy) pixel-wise instead of image-wise. 
We performed this step for $1000$ iterations, with learning rate $1.0$ and batch size 8, aggregating the gradient of 2 training episodes, as in~\cite{gidaris2018dynamic}. After the meta learning stage, the method includes new classes in the FSL steps by weight imprinting, that we implemented with MAP, as for WI.%  We underline that, since this method is not trained after the base step, the second learning stage has been performed once after the training on the base dataset.}

Rethinking FSL \cite{tian2020rethinking} (RT), refines the model during the base step by using self-distillation and fine-tunes the classifier on the FSL step. In particular, after the base step a copy of the model is stored and provides the target of the self-distillation loss, to the current model. This training phase uses the same hyperparameters of the base one. %after the base step the current model is saved performing multiple training rounds where the model is train the model in the base step with their self-distillation loss, applying it pixel-wise. \massi{
%after training the model in the base step, we perform another round of training, with the same hyperparameters of the base step but applying a self-distillation loss (pixel-wise), where the target are provided by a copy of the network at the end of the previous round. 
 We stopped after one additional training round %of self-distillation 
because we did not see clear improvements using more rounds at the expense of a longer training time. For iFSS, we applied the self-distillation loss pixel-wise.
For the FSL steps, we trained the classifier for new classes starting from random weights and freezing the rest of the network. We multiplied the learning rate by 10 \wrt the Sec~\ref{sec:training-protocol} on the FSL step, since this improved the performance on both datasets.

Adaptive Masked Proxies \cite{siam2019adaptive} (AMP) has been implemented following details in \cite{siam2019adaptive} uses a standard linear classification layer and, %following Eq.~1b of \cite{siam2019adaptive}, it uses 
an L2-normalized MAP features % of the features extracted with MAP 
as classifier for the new classes. 
% \massi{After initializing the weights of the new classes with normalized MAP, it continuously updates them if new images whenev normalizes the features obtained with masked average pooling. The classifier weights are updated following Eq.~2 of \cite{siam2019adaptive}, setting $\alpha$ equals to $0.25$. \fabio{Come adattato su vecchie.}}
We adapted AMP to work on both old and new classes using all the available annotations in the FSL dataset. In particular, as proposed by \cite{siam2019adaptive} for continuous segmentation, we update the classifier weights for all the old classes appearing in the new dataset by computing a moving average %, as in Eq.~2 of \cite{siam2019adaptive}, 
with update rate $\alpha=0.25$.

For Semantic Projection Network \cite{xian2019spnet} (SPN) we follow the implementation provided by the authors, using the combination of word2vec \cite{mikolov2013distributed} and fastText \cite{joulin2016fasttext} as class embeddings, using them direclty as classifier weights. %as in \cite{xian2019spnet}. 
The method has no specific hyperparameters and we adapt it to \SET\ by not retaining the old datasets in the learning steps.

We implemented the three incremental learning methods, Learning without Forgetting \cite{li2017learning} (LwF), Incremental Learning Techniques \cite{michieli2019incremental} (ILT), and Modeling the Background \cite{cermelli2020modeling} (MiB), following the code provided by \cite{cermelli2020modeling}. As regularizer, LwF and ILT apply a standard cross-entropy loss using the old network predictions as target, and ILT imposes an additional L2 constraint on the output of the backbone (\ie the Resnet-101). MiB uses the revised cross-entropy and distillation losses as well as the classifier weights initialization for new classes. The weight of the distillation losses is $100$ for LwF, $100$ on both the L2 and the cross-entropy for ILT, and $10$ for MiB. %For all methods, we use the few-shot images in place of the many-shots datasets of standard incremental learning. 

Finally, for our model we set $\lambda$ to $10$ for all settings. We recall that for all the baseline we report in the paper, we used the same training protocol and architectures of \ours. 

\begin{table}[t]
    \centering
    \begin{tabular}{c|p{5cm}}
         \textbf{split}  &  \textbf{classes} \\ \hline
         5-0  &  aeroplane, bicycle, bird, boat, bottle \\
         5-1  &  bus, car, cat, chair, cow \\
         5-2  &  table, dog, horse, motorbike, person \\
         5-3  &  plant, sheep, sofa, train, tv-monitor \\
    \end{tabular}
    \vspace{4pt}
    \caption{Pascal-VOC class split.} \label{tab:voc-split}
    \vspace{-4pt}
\end{table}

\begin{table}[t]
    \centering
    \begin{tabular}{p{1cm}|p{6.5cm}}
         \textbf{split}  &  \textbf{classes} \\ \hline
         20-0  &  person, airplane, boat, parking meter, dog, elephant, backpack, suitcase, sports ball, skateboard, wine glass, spoon, sandwich, hot dog, chair, dining table, mouse, microwave, refrigerator, scissors \\
         20-1  &  bicycle, bus, traffic light, bench, horse, bear, umbrella, frisbee, kite, surfboard, cup, bowl, orange, pizza, couch, toilet, remote, oven, book, teddy bear \\
         20-2  &  car, train, fire hydrant, bird, sheep, zebra, handbag, skis, baseball bat, tennis racket, fork, banana, broccoli, donut, potted plant, tv, keyboard, toaster, clock, hair drier \\
         20-3  &  motorcycle, truck, stop sign, cat, cow, giraffe, tie, snowboard, baseball glove, bottle, knife, apple, carrot, cake, bed, laptop, cell phone, sink, vase, toothbrush \\
    \end{tabular}
    \vspace{4pt}
    \caption{COCO class split.} \label{tab:coco-split}
    \vspace{-4pt}
\end{table}

\subsection{Dataset class splits}
We split both Pascal-VOC and COCO in 4 folds, following previous works in semantic segmentation \cite{nguyen2019feature, wang2019panet, zhang2019canet, shaban2017one, rakelly2018few}. Table \ref{tab:voc-split} reports the detailed class folds for Pascal-VOC, \rev{taken from \cite{shaban2017one},} and Table \ref{tab:coco-split} the ones for the COCO dataset, \rev{taken from \cite{nguyen2019feature}}.

\begin{figure}
    \centering
    \begin{subfigure}{0.45\textwidth}
        \includegraphics[width=\textwidth]{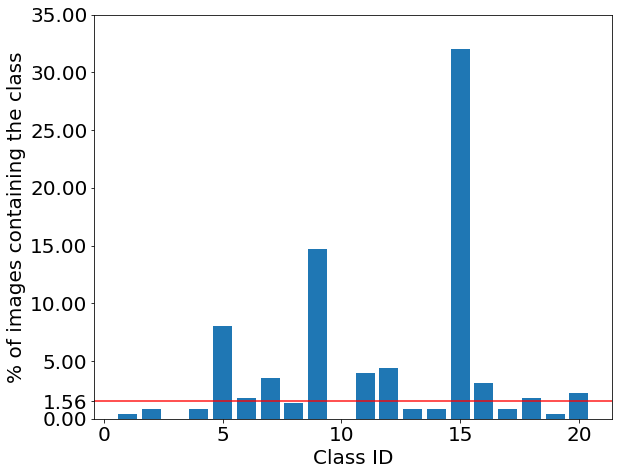}
        \caption{VOC} 
    \end{subfigure}
    \begin{subfigure}{0.45\textwidth}
        \includegraphics[width=\textwidth]{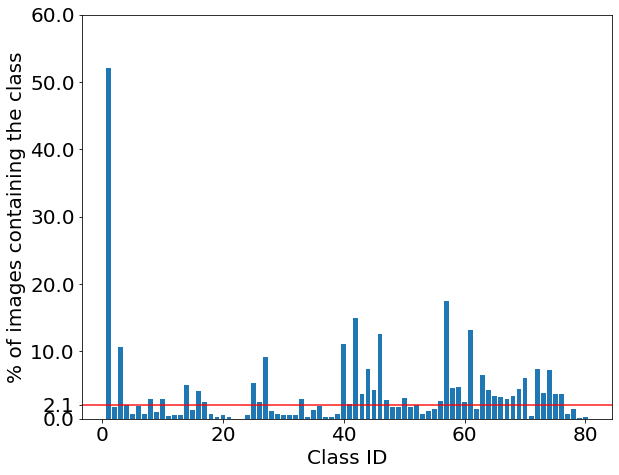}
        \caption{COCO} 
    \end{subfigure}
    \vspace{5pt} \caption{Percentage of images containing the old class in the 5-shot setting datasets. We note that class \textit{person} has class-ID 15 on VOC and 1 on COCO. The red line represents the median over all classes.}
    \label{fig:perc_img}
\end{figure}

\rev{
\section{Influence of old classes annotations in iFSS}
The few-shot learning steps (FSL) in our benchmark consider a dataset with 1, 2, or 5 images for each new class, {randomly} sampled from the set of images containing at least one pixel of that class, but \textit{without} imposing any constraint about the presence of old classes. However, differently from \cite{cermelli2020modeling}, the few-shot datasets provide annotation for all available pixels, both for new and old classes.
In this section, we first analyze the frequency with which old classes appears in few-shot learning steps, showing that they co-occurs rarely with new classes.
Then, we compare the results of the settings using (non-strict IL) and not using (strict IL) old classes annotations.

\subsection{Frequency of old classes in few-shot learning datasets}
Fig.\ref{fig:perc_img} reports the percentage of images per old class averaged on all folds of the 5-shot settings.
From the figure, we note that old classes rarely co-occur when learning new classes: the median is 1.56\% of images per old class on VOC and 2.1\% on COCO. The only exception is the \textit{person} class that frequently appears in the few-shot dataset: in 32\% of images in VOC and in 52\% in COCO. Moreover, we note that many classes never appear with new classes, both in VOC, such as classes 4 (\textit{boat}) and 10 (\textit{cow}), and in COCO, \eg classes 22 (\textit{bear}) and 23 (\textit{zebra}).

\begin{table*}[t]
    \centering
    \setlength{\tabcolsep}{3pt} % Default value: 6pt
    \resizebox{\linewidth}{!}
    {\begin{tabular}{c|c|ccc|ccc|ccc||ccc|ccc|ccc}
    \multicolumn{2}{c|}{} & \multicolumn{9}{c||}{\textbf{VOC-SS}} & \multicolumn{9}{c}{\textbf{COCO-SS}}  \\
    \multicolumn{2}{c|}{} & \multicolumn{3}{c}{\textbf{1-shot}} & \multicolumn{3}{c}{\textbf{2-shot}} & \multicolumn{3}{c||}{\textbf{5-shot}} & \multicolumn{3}{c}{\textbf{1-shot}} & \multicolumn{3}{c}{\textbf{2-shot}} & \multicolumn{3}{c}{\textbf{5-shot}} \\ \hline
    Method & Strict & mIoU-B & mIoU-N	 & HM	 & mIoU-B & mIoU-N	 & HM & mIoU-B & mIoU-N	 & HM & mIoU-B & mIoU-N	 & HM	 & mIoU-B & mIoU-N	 & HM & mIoU-B & mIoU-N	 & HM  \\ \hline     \rowcolor{rowColor}
    FT               &        & 58.2 &	 9.7 & 16.6	& 59.1 &	19.6 &	29.5 &	55.8 & 29.5 &	38.6                        & 41.2&	 4.1&	 7.5&	41.5&	 7.3&	12.4&	41.6&	12.3 &	19.0 \\ 
    FT        	     & \cmark & 55.0 &	10.2 & 17.2	& 55.5 &	19.2 &	28.5 &	43.7 & 26.8 &	33.2                        & 35.3&	 4.5&	 8.0&	32.8&	 7.4&	12.1&	26.9&	11.1&	15.7 \\ \rowcolor{rowColor}
    WI \cite{qi2018low}              &        & \bb{62.6} &	15.4 & 24.8	& 63.2 &	19.2 &	29.4 &	63.2 & 21.7 &	32.3                    & \bb{43.8}&	 6.9&	11.9&	44.2&	 7.9&	13.5&	43.6&	 8.7 &	14.6 \\ 
    WI \cite{qi2018low}      	     & \cmark & \br{62.6} &	15.4 & 24.8	& 63.2 &	19.2 &	29.4 &	63.2 & 21.7 &	32.3                    & \br{43.8}&	 6.9&	11.9&	\br{44.2}&	 7.9&	13.5&	43.6&	 8.7 &	14.6 \\ \rowcolor{rowColor}
    SPN  \cite{xian2019spnet}              &        & 59.8 &	16.3 & 25.6	& 60.7 &	\bb{26.3} &	\bb{36.7} &	58.3 & \bb{33.4} &	42.4            & 43.5&	 6.7&	11.7&	43.7&	10.2&	16.5&	43.7&	\bb{15.6} &	\bb{22.9} \\ 
    SPN  \cite{xian2019spnet}      	     & \cmark & 56.3 &	16.4 & 25.4	& 57.0 &	25.3 &	35.1 &	48.6 & 30.2 &	37.3                        & 38.1&	 7.0&	11.8&	37.0&	10.4&	16.3&	33.2&	15.1 &	20.8 \\ \rowcolor{rowColor}
    MIB \cite{cermelli2020modeling}             &        & 61.0 &	 5.2 &  9.6	& \bb{63.5} &	12.6 &	21.1 &	\bb{64.9} & 28.1 &	39.2                & \bb{43.8}&	 3.5&	 6.5&	\bb{44.4}&	 6.0&	10.6&	\bb{44.7}&	11.9 &	18.8 \\ 
    MIB \cite{cermelli2020modeling}      	     & \cmark & 61.0 &	 6.0 & 11.0	& \br{63.5} &	13.7 &	22.5 &	\br{64.9} & 29.4 &	40.4                & \br{43.7}&	 4.2&	 7.7&	\br{44.2}&	 7.1&	12.3&	\br{44.4}&	13.8 &	21.1 \\ \rowcolor{rowColor}
    PIFS             &        & 60.8 &	\bb{18.5} & \bb{28.4}	& 60.5 &	\bb{26.3} &	\bb{36.7} &	60.0 & 33.2 &\bb{42.8}  & 40.8&	 \bb{8.2}&	\bb{13.6}&	40.9&	11.1&	\bb{17.5}&	42.8&	\bb{15.7} &	\bb{23.0} \\ 
    PIFS      	     & \cmark & 59.1 &	\br{18.2} & \br{27.9}	& 58.8 &	26.1 &	36.2 &	57.2 & 32.5 &	41.5            & 34.9&	 \br{8.9}&	14.2&	34.6&	11.7&	17.4&	32.6&	15.6 &	21.1 \\ 
    PIFS*	    & \cmark & 60.3 &	18.0 & 27.7	& 60.3 &	\br{26.3} &	\br{36.6} &	59.5 & \br{33.0} &	\br{42.5}       & 38.8&	 8.8&	\br{14.4}&   39.2&	\br{11.8}&	\br{18.1}&	38.4&	\br{16.1} &	\br{22.6} \\ 
    \end{tabular}}
    \vspace{-2pt} \caption{Performance in strict and non-strict incremental learning on single-step settings. In bold-red the best method in strict-IL scenario. In bold-blue, the best method in non strict-IL. PIFS* uses the revised classification loss proposed by MIB \cite{cermelli2020modeling}.} \label{tab:strict}
    \vspace{-15pt}
\end{table*}

\subsection{Comparison between iFSS in strict and non-strict settings}
Tab.~\ref{tab:strict} reports the comparison among the strict and non-strict setting of some indicative methods, FT, WI \cite{qi2018low}, SPN \cite{xian2019spnet}, MIB \cite{cermelli2020modeling} and PIFS, evaluating the impact of the background shift on them. We also report PIFS*, which uses the revised classification loss proposed by MIB \cite{cermelli2020modeling} to deal with the background shift.
First, we note that WI obtains the same results in the two settings since it is not affected by the annotation on old classes and it only uses new classes' pixels for generating the classifier weights. 
Differently, FT and SPN, suffer the background shift, as indicated by the large decrease in mIoU-B on all setting. 
MIB, being designed to solve deal with the background shift, even improves its performance, obtaining similar results in mIoU-B and improving its performance on mIoU-N. 
Finally, we note that PIFS is robust to the background shift on VOC but it decrease in performance on mIoU-B on COCO. Moreover, it obtains outstanding performance on new classes, constantly outperforming the competitors on mIoU-N.
Introducing the cross-entropy loss of MiB \cite{cermelli2020modeling} in PIFS, it notably improves the results on old classes, alleviating the background shift. We remark that introducing the loss of \cite{cermelli2020modeling} is straightforward, since the choice of classification loss is independent from the prototype-learning and the distillation loss of PIFS.
}

\begin{figure}
  \centering
\begin{subfigure}{0.3\textwidth}
  \centering
  \includegraphics[width=\linewidth]{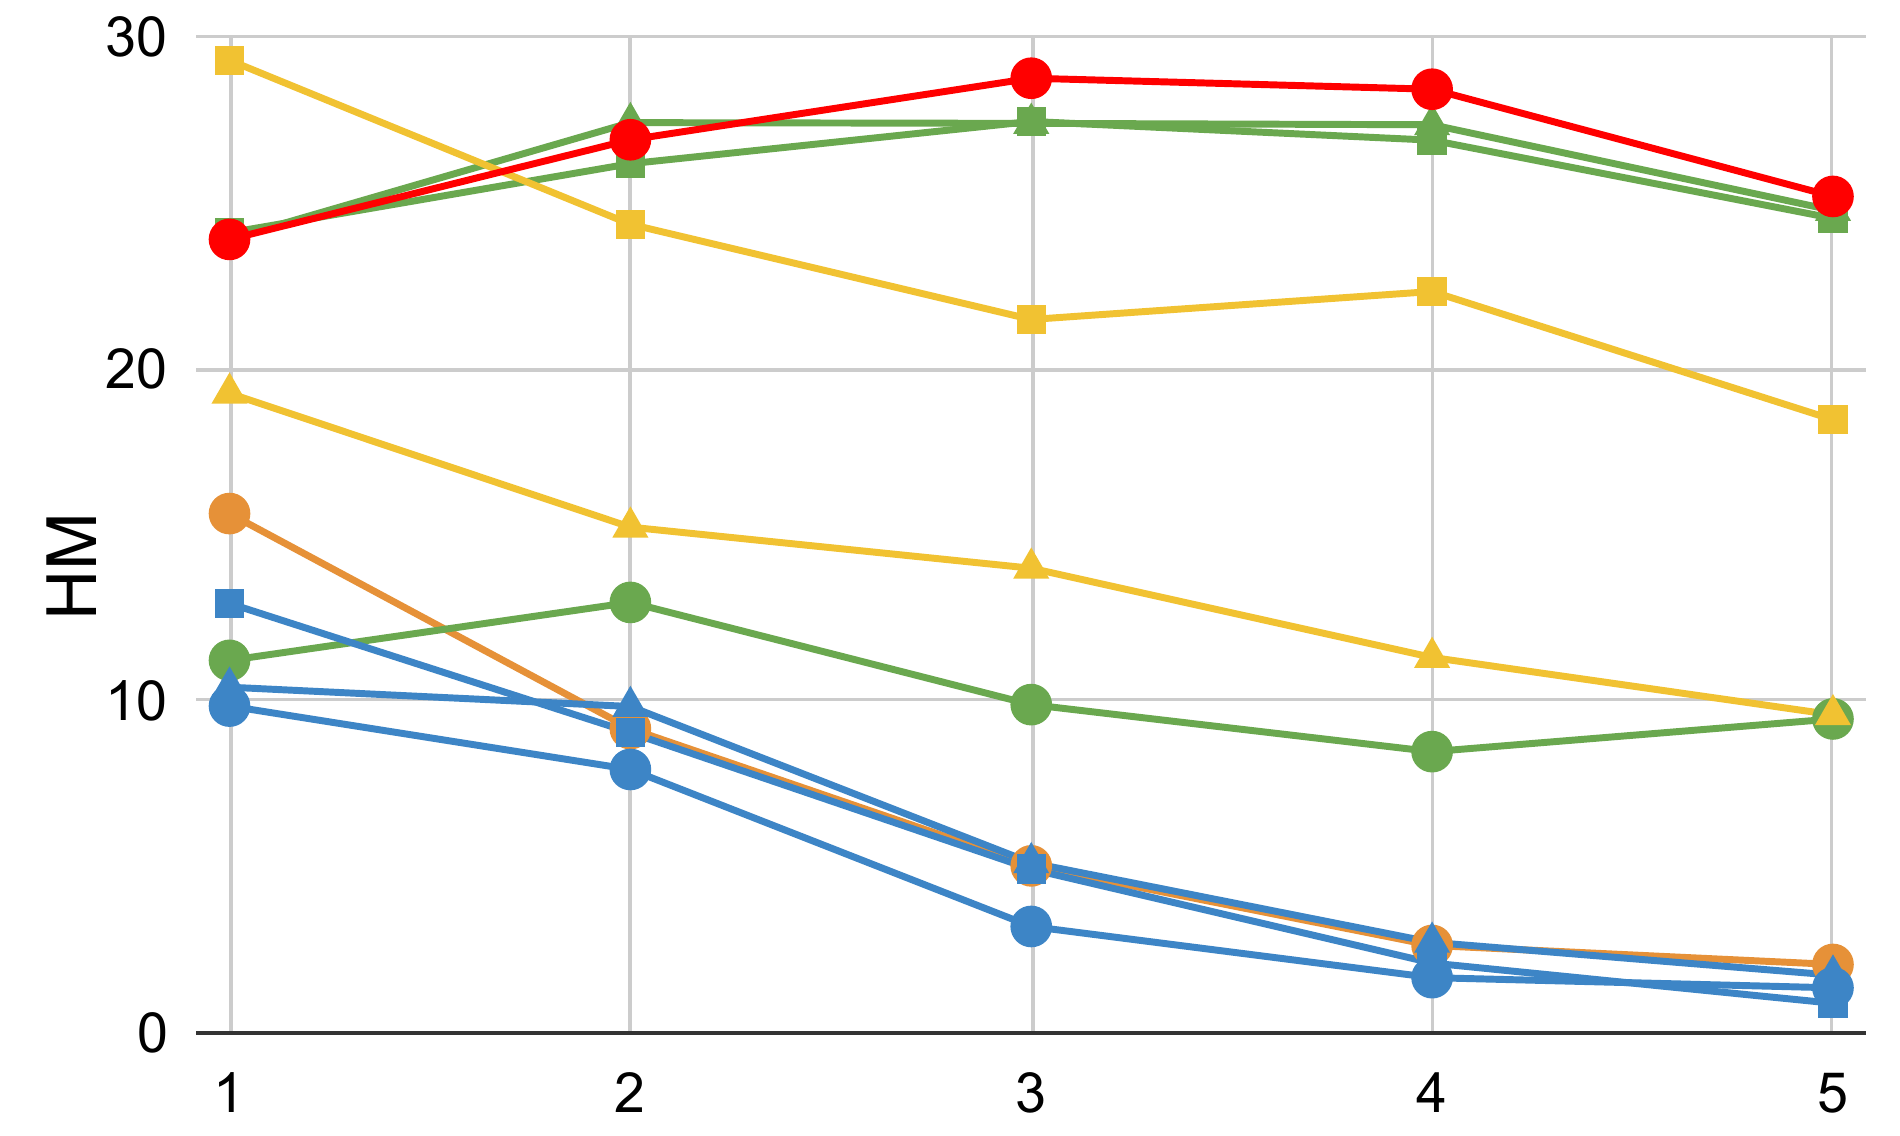}
  \caption{VOC 1-shot}
  \vspace{-5pt}
\end{subfigure}%
\begin{subfigure}{0.3\textwidth}
  \centering
  \includegraphics[width=\textwidth]{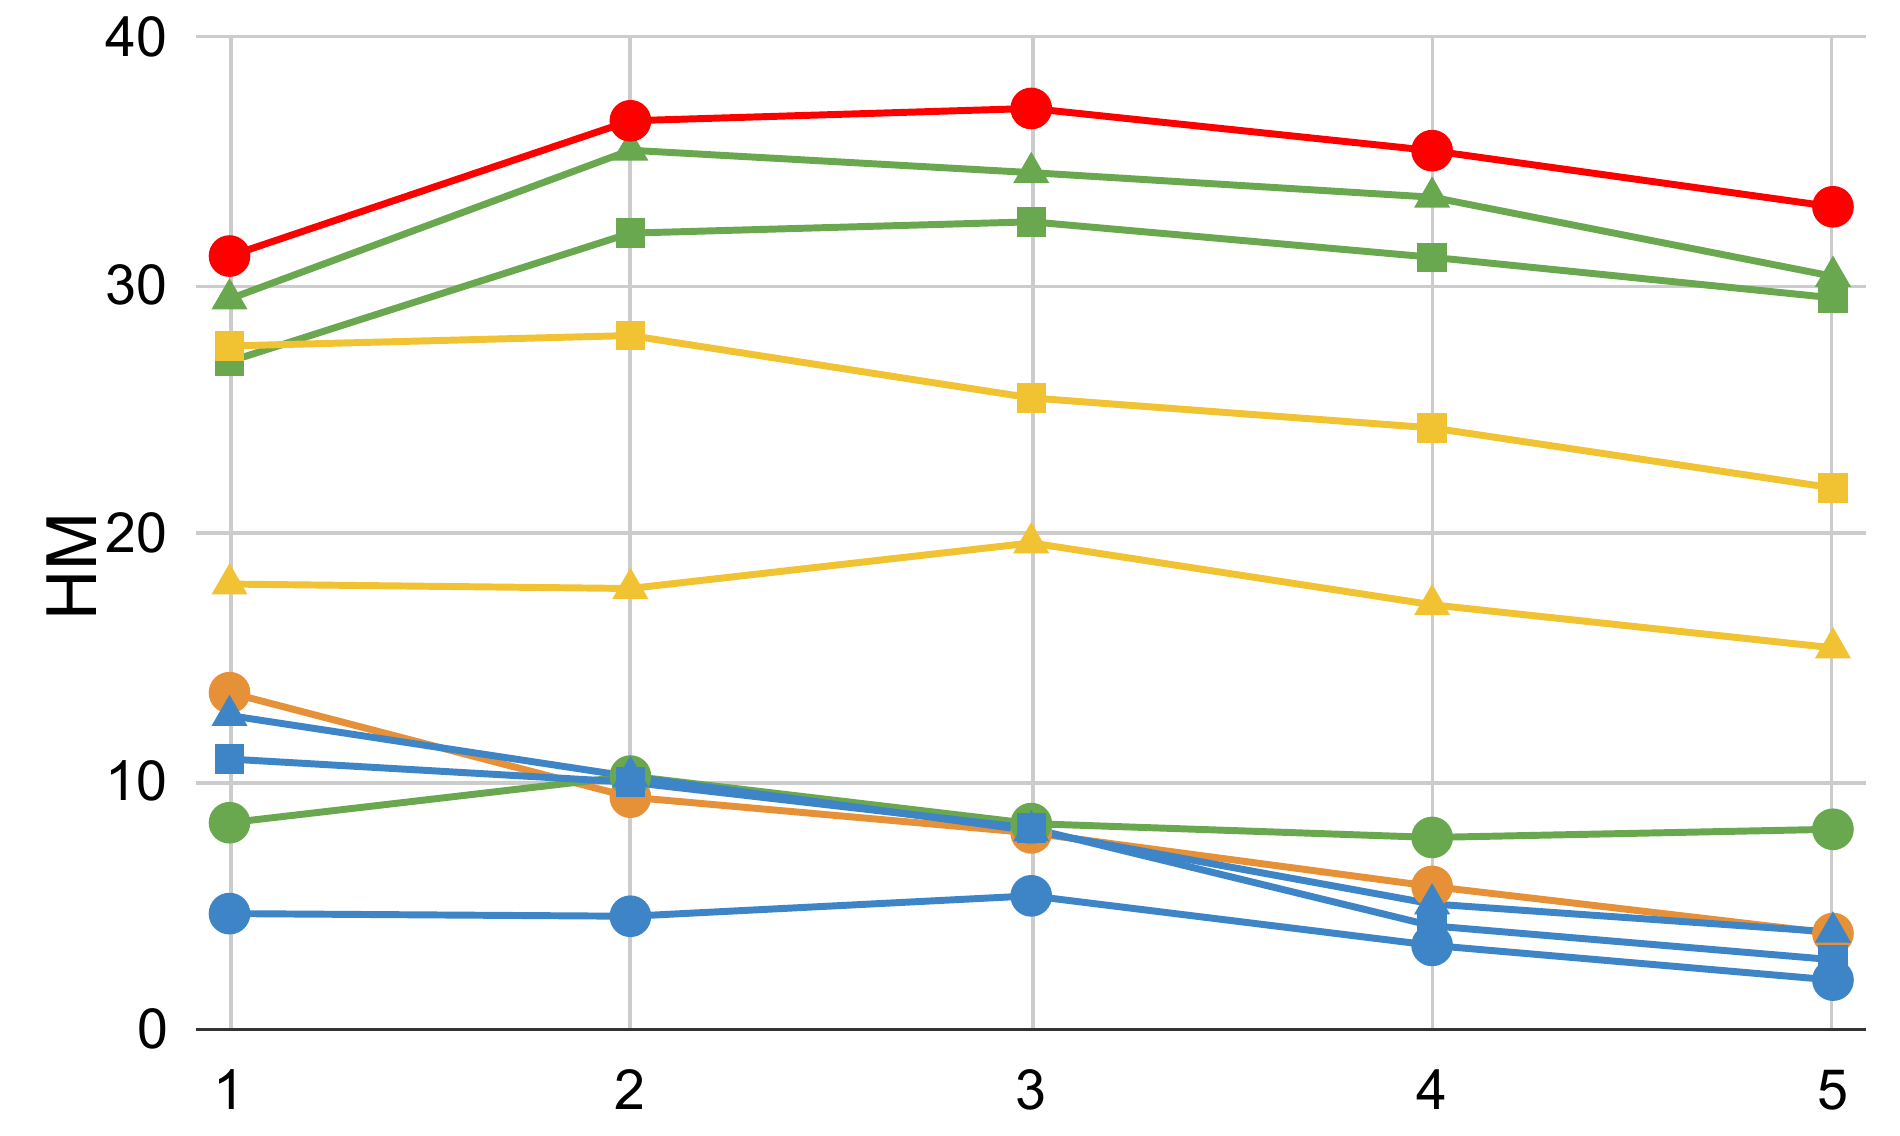}
  \caption{VOC 2-shot}
    \vspace{-5pt}
\end{subfigure}%
\begin{subfigure}{0.3\textwidth}
  \centering
  \includegraphics[width=\textwidth]{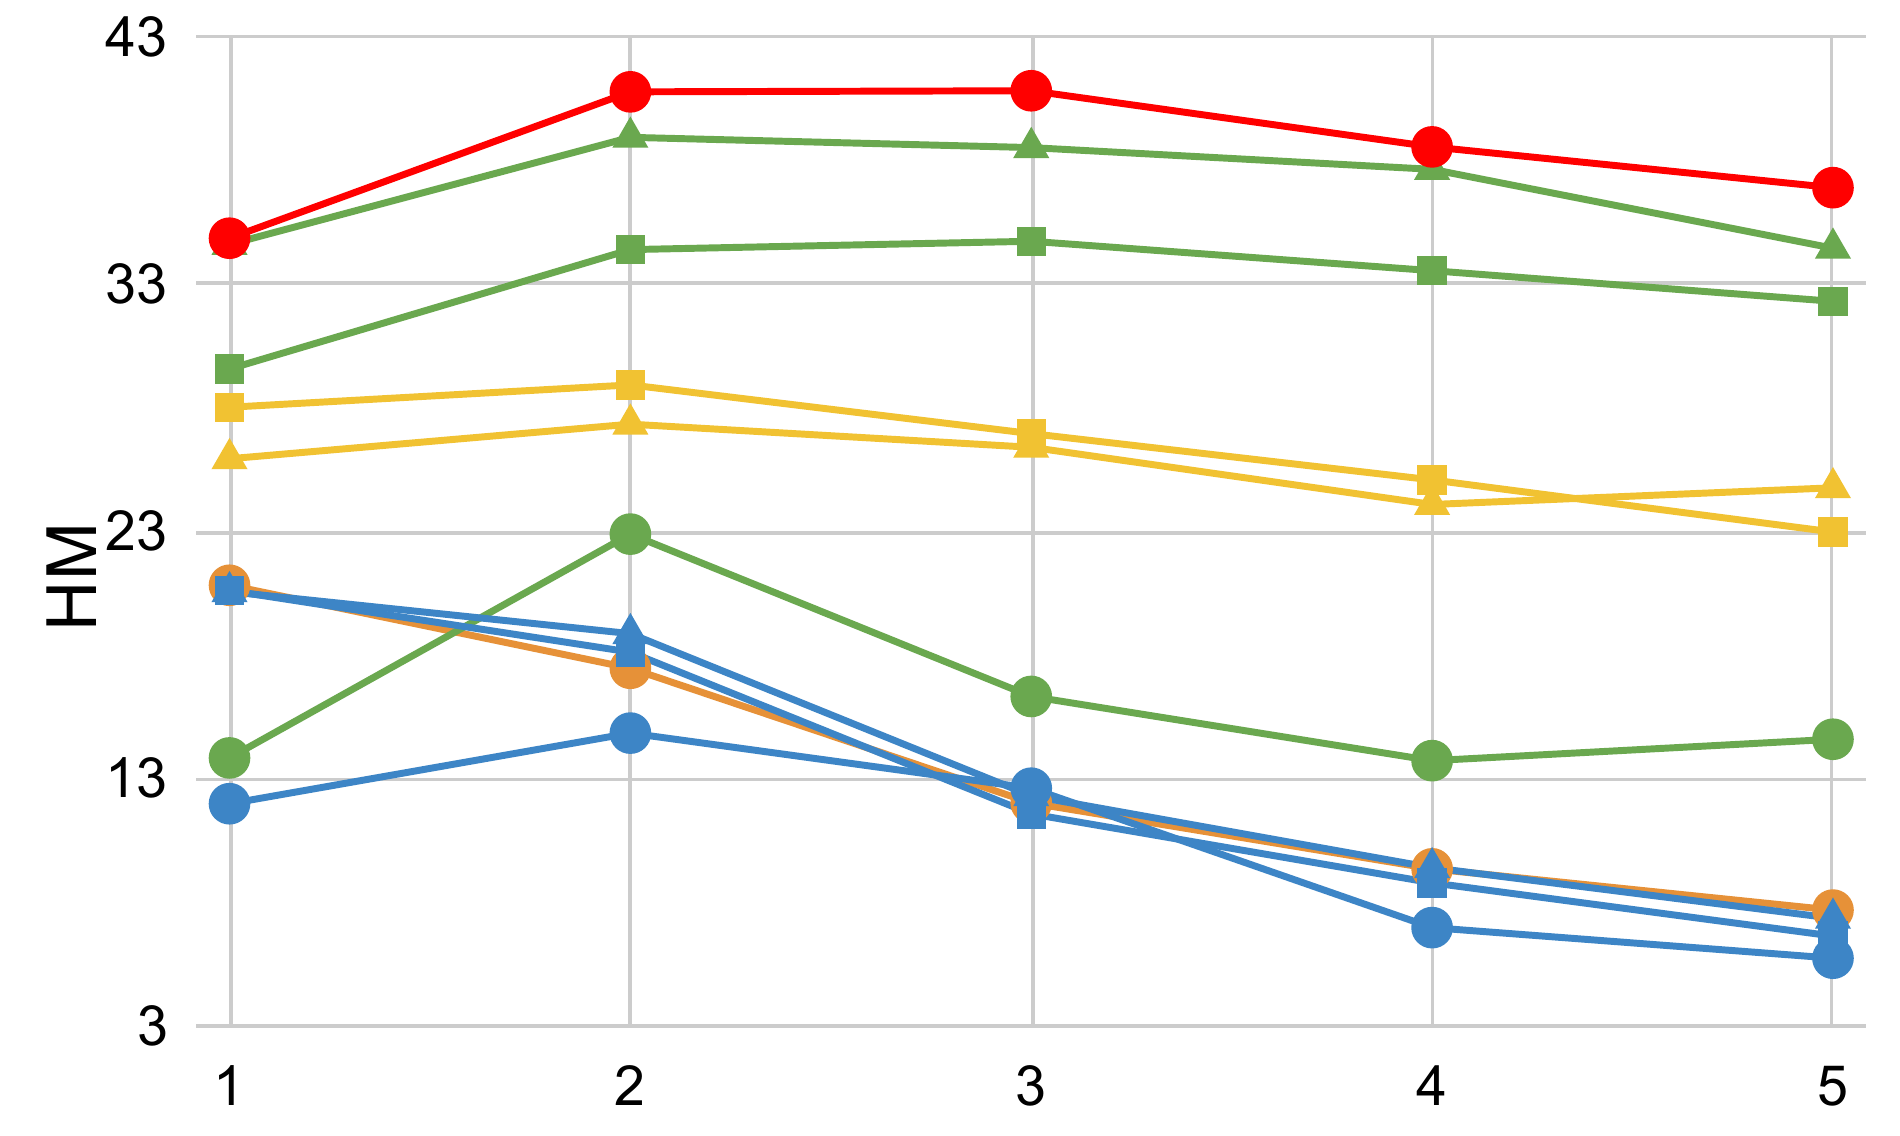}
  \caption{VOC 5-shot}
    \vspace{-5pt}
\end{subfigure}
\begin{subfigure}{0.056\textwidth}
  \centering
  \includegraphics[width=\textwidth]{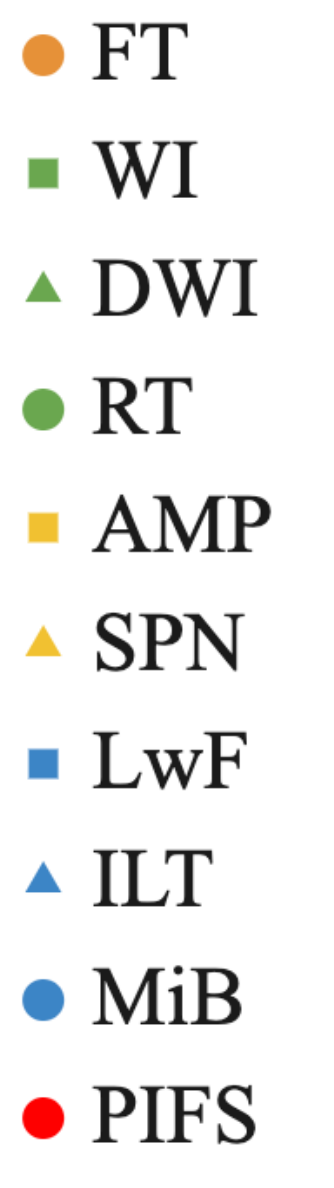}
    \vspace{2pt}
\end{subfigure}

\begin{subfigure}{0.3\textwidth}
  \centering
  \includegraphics[width=\textwidth]{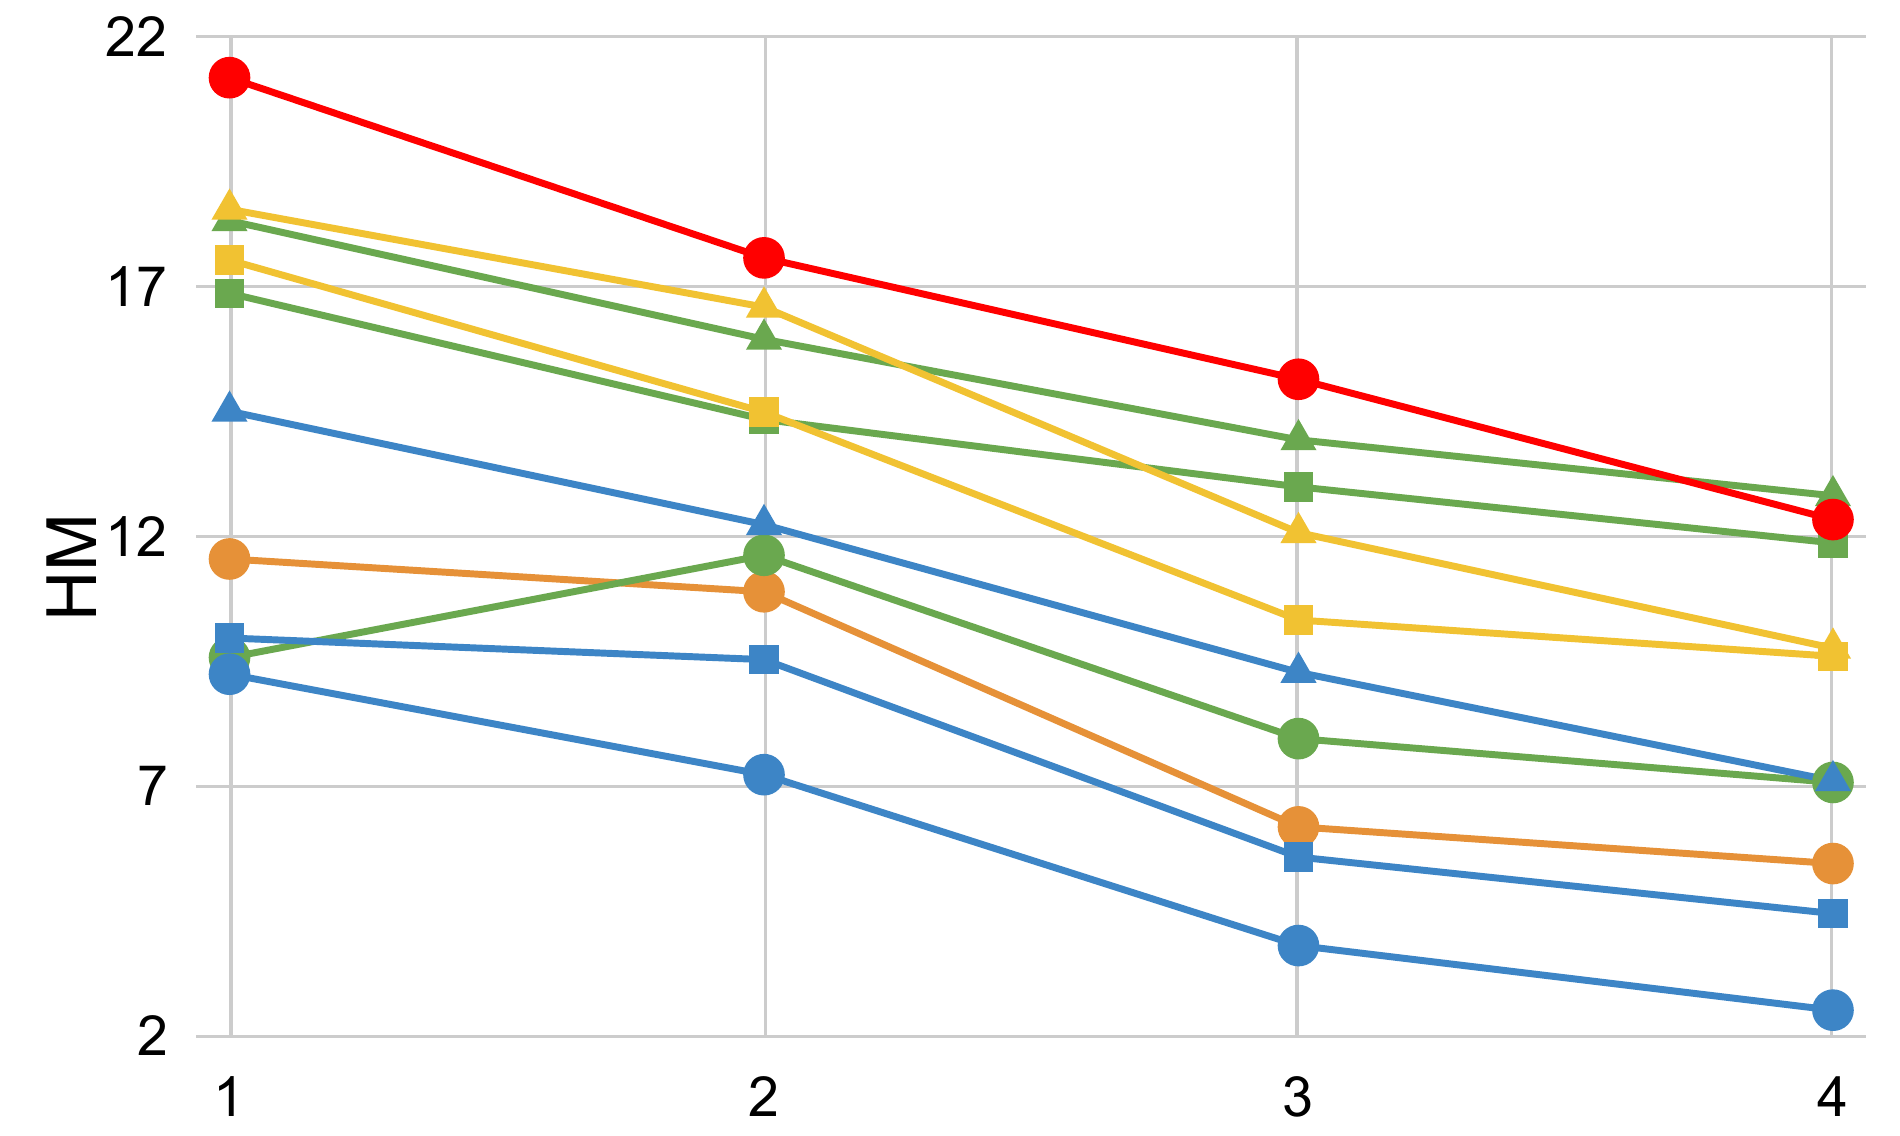}
  \caption{COCO 1-shot}
\end{subfigure}
\begin{subfigure}{0.3\textwidth}
  \centering
  \includegraphics[width=\textwidth]{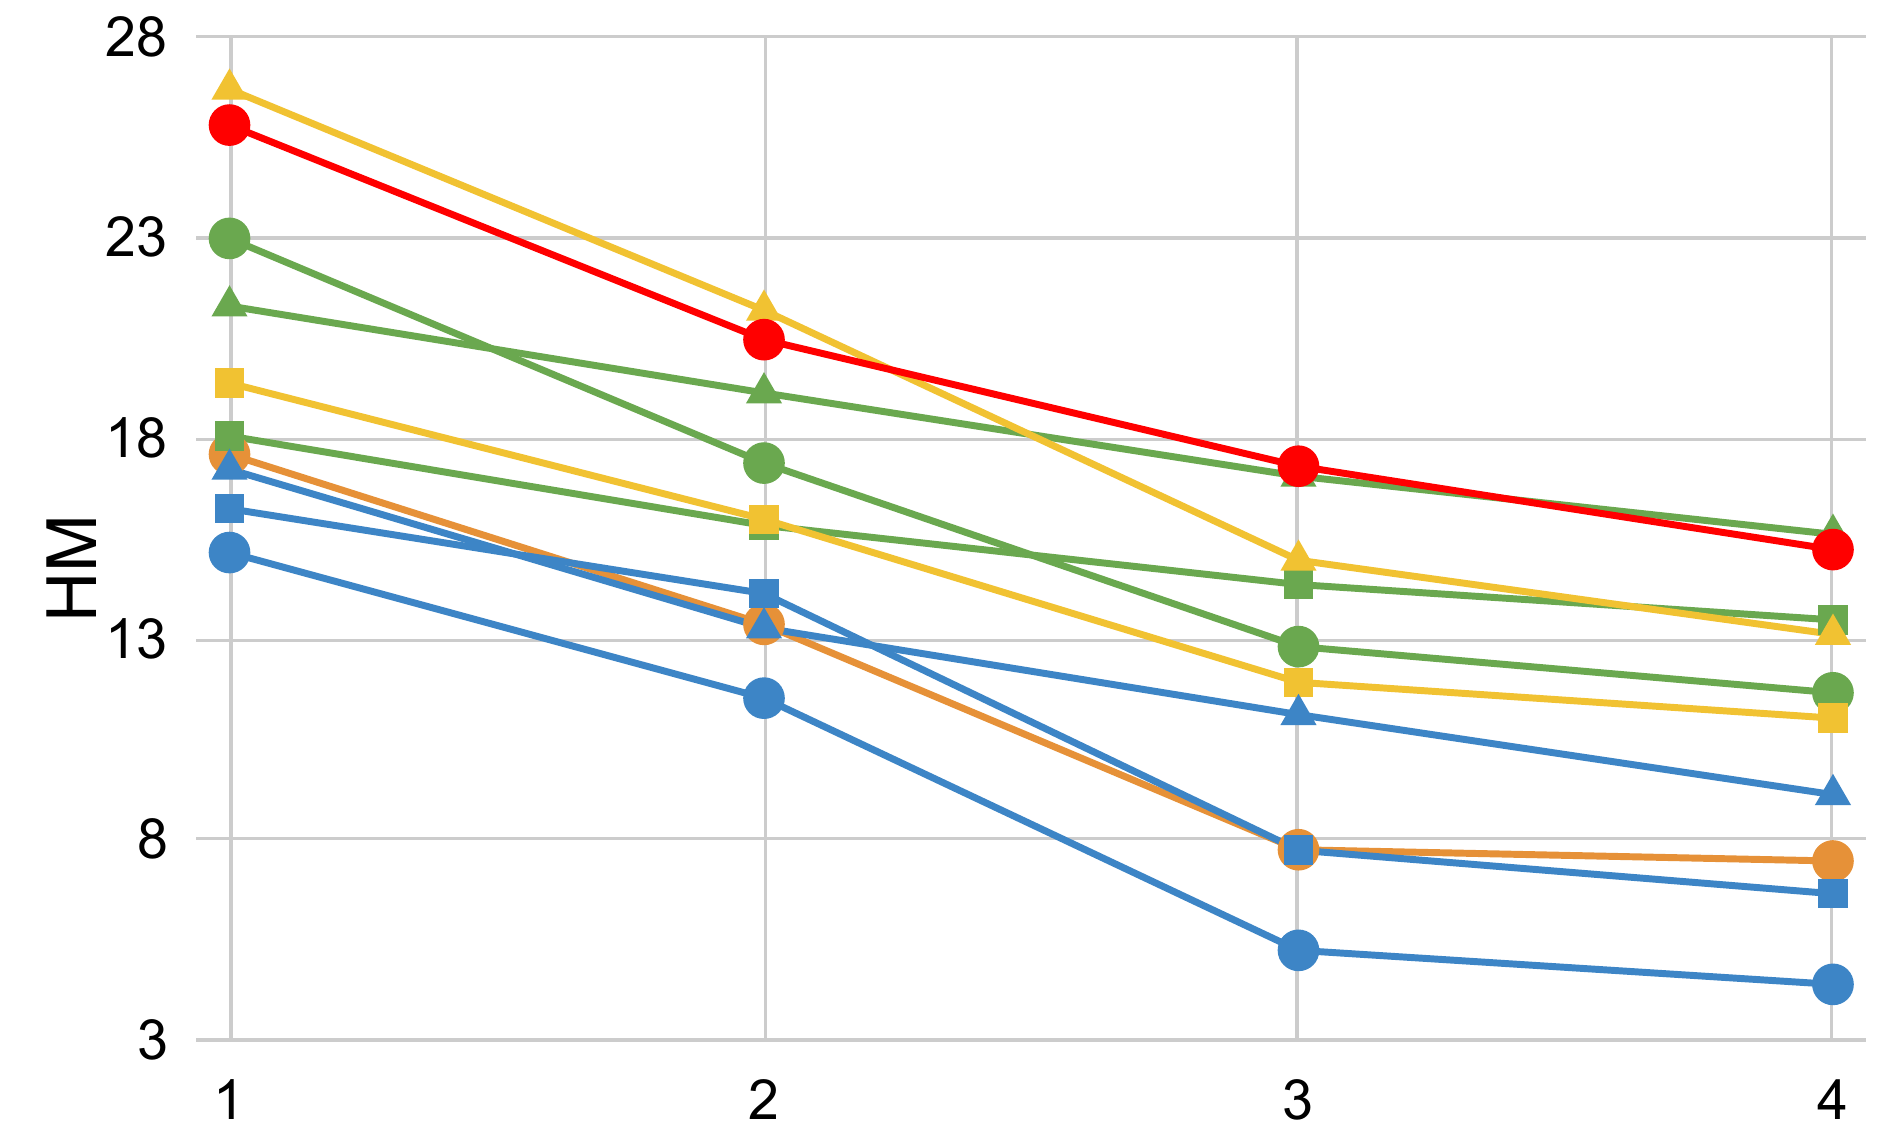}
  \caption{COCO 2-shot}
\end{subfigure}
\begin{subfigure}{0.3\textwidth}
  \centering
  \includegraphics[width=\textwidth]{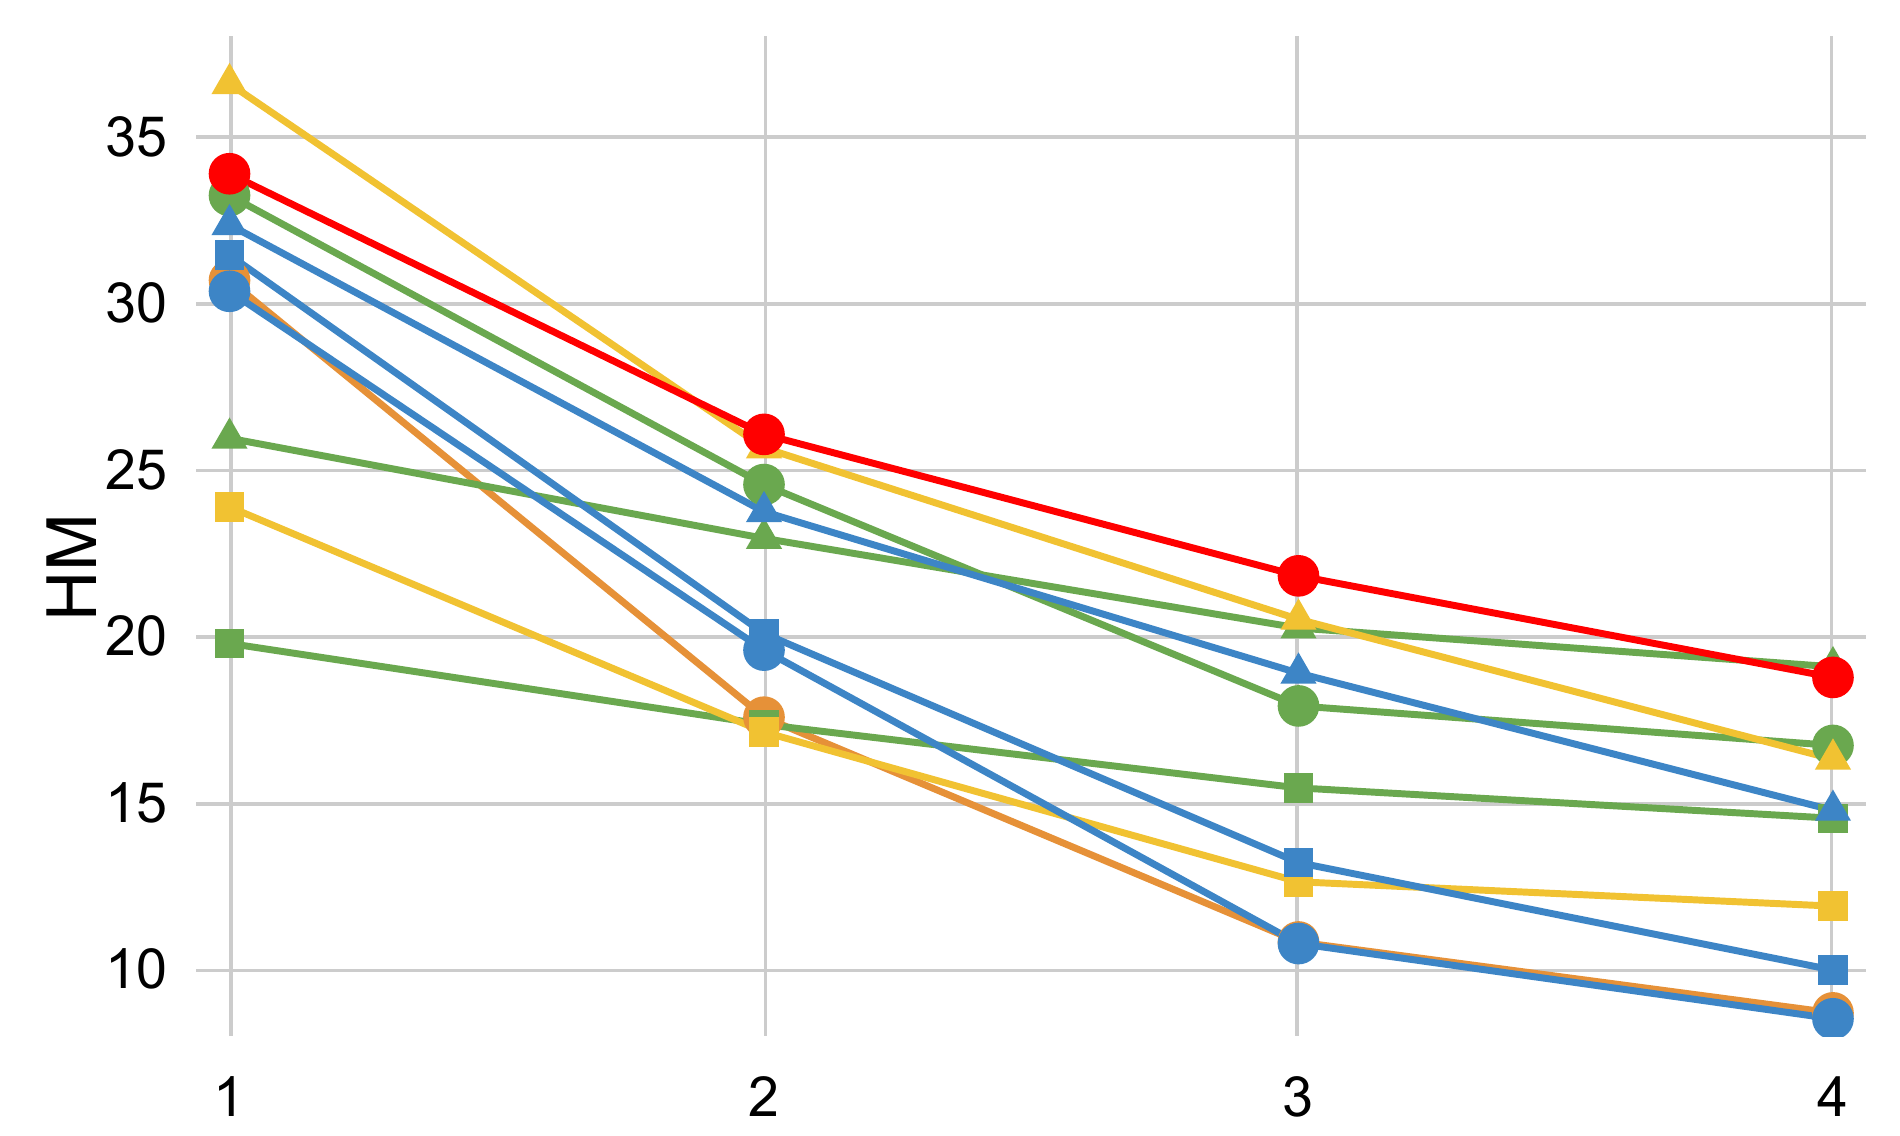}
  \caption{COCO 5-shot}
\end{subfigure}
\begin{subfigure}{0.056\textwidth}
  \centering
  \includegraphics[width=\textwidth]{fig/plot22/legend.pdf}
  \vspace{2pt}
\end{subfigure}
\vspace{2pt}
\caption{\SET\ results on the sequential addition of new class. Every column is a new step.}
\vspace{-10pt}
\label{fig:multi-step}
\end{figure}

\section{Additional results}
\vspace{4pt}

\subsection{Detailed results step-by-step}
We report the results for every incremental step on the VOC-MS and COCO-MS settings in \figref{fig:multi-step}. For every incremental step, we report the harmonic mean (HM) between the mIoU on base ($\set C^0$) and new ($\set C^t \backslash \set C^0$) classes.

From the results, we note that fine-tuning (orange), RT \cite{chen2017rethinking} (green, circle), and incremental learning methods \cite{cermelli2020modeling, michieli2019incremental, li2017learning} (blue) obtain the worst performance on all settings. We argue that this is due to: i) not exploiting prototype learning, failing to correctly initialize and represent the new classes, and ii) not dealing with the non-\textit{i.i.d.} data, as demonstrated by the poor performances obtained on VOC when few images are provided (1- and 2-shot settings). 
On the other hand, methods that perform prototype learning, %do not perform training in the incremental steps, 
such as few-shot classification methods \cite{qi2018low, gidaris2018dynamic} (green) and AMP \cite{siam2019adaptive} (yellow, square), show a better trade-off between learning and forgetting. In particular, WI \cite{qi2018low} and DWI \cite{gidaris2018dynamic} achieve good performance on VOC, being close to \ours\ (red) especially on the 1-shot setting. However, we note that on VOC 5-shot and COCO, \ours\ obtains better performances since it fine-tunes the network on the few-shot data, obtaining a better representation while avoiding overfitting. AMP \cite{siam2019adaptive}, differently, is outperformed by \ours, remarking that it is essential to update the network representation and not only the prototypes during the FSL steps.
Finally, SPN \cite{xian2019spnet} (yellow, triangle) achieves good performance on the initial steps of COCO-MS 2- and 5-shot settings, even surpassing \ours. However, after only one (5-shot) or two (2-shot) learning steps its performances degrade and it is surpassed by \ours. This demonstrates that \ours\ improves the representation for new class pixels while better dealing with forgetting and non-\textit{i.i.d.} data, even without using external knowledge.
Overall, \ours\ is consistently the best on every dataset and shot.

\subsection{Detailed results for each split}
Due to space constraints, in the main paper we report the average results across the 4 splits of classes of each dataset. % in which we split the two datasets. % classes. 
Here, we report the detailed results in all folds separately, measuring them as the mIoU on base (\textit{mIoU-B}) and new (\textit{mIoU-N}) classes, and their harmonic mean (\textit{HM}). %Table \ref{tab:voc-split} reports the class folds for Pascal-VOC, and Table \ref{tab:coco-split} the ones for the COCO dataset. 

\myparagraph{Pascal VOC.} We report the results for Pascal-VOC with only one few-shot learning step (VOC-SS) on Tab.~\ref{tab:voc-ss-1} for 1-shot, on Tab.~\ref{tab:voc-ss-2} for 2-shot, and on Tab.~\ref{tab:voc-ss-5} for 5-shot. The results on each fold are consistent with their average. %, with 
%From the tables we can see that 
\ours\  is effective on all the VOC folds, being always the best on 1-shot, and always the best or second best on 2-shot scenario, in terms of HM. Moreover, we note that SPN is the second best on both 2-shot and 5-shot scenarios, on all folds.
On 5-shot scenario incremental learning methods become competitive to \ours, being ILT the best on 5-0 ($+1.7$\% HM \wrt \ours) and LwF on 5-1 ($+3.4$\% HM \wrt \ours). However the improvement of these methods is not consistent in other folds (\eg 5-3, where \ours\ improves ILT of 5.1\% in HM), %or settings (\ie 1-shot and 2-shot), 
obtaining an average performance lower than \ours. %  and SPN. 

Tables \ref{tab:voc-ms-1}, \ref{tab:voc-ms-2}, and \ref{tab:voc-ms-5} report the results (averaged per FSL step) for the multi step scenario (VOC-MS), for the 1, 2, and 5 shot respectively. We remark that this setting is particularly challenging since methods are provided only with 1, 2 or 5 images of the same class to train, resulting in very unbalanced and non-\textit{i.i.d} set. 
In this setting, \ours\ obtains the best results on 5-1, 5-2, and 5-3, in both 1, 2, and 5-shot setting, achieving the second best results on 5-0 on 2 and 5-shot. We note that methods obtaining excellent performance on VOC-SS struggle on this scenario. In particular, SPN performances are lower than \ours\ of 15\% HM on average, while incremental learning methods are not able to learn new classes properly, performing close to standard fine-tuning. %, \ie 30\% HM worse than \ours\ on average.
On the other hand, DWI and WI are effective on this scenario, since they can integrate new classes without forgetting previous knowledge. DWI is the second best method on both 1, 2, and 5-shot, being the best on the 5-0 fold. However, \ours\ still outperforms it by $0.5$\% HM on 1-shot, $2.1$\% HM on 2-shot, and $1.7$\% HM on 5-shot.

\myparagraph{COCO.} The results for COCO-SS are reported on tables \ref{tab:coco-ss-1} (1-shot), \ref{tab:coco-ss-2} (2-shot), and \ref{tab:coco-ss-5} (5-shots). From the tables we can see that \ours\ is consistently best or second best on every shot and fold. It achieves nearly 1\% HM more than the second best method in 1-shot ($13.6$\% \wrt DWI $12.8$\%) and in 2-shot ($17.5$\% \wrt SPN $16.5$\%). %We can see that this improvement is consistent across all the folds.
Differently, on 5-shot SPN achieves comparable performance to \ours, \ie $22.9$\% vs $23.0$ HM. From the detailed results on the folds we can see that while SPN obtains better results on 20-0 and 20-1 ($+1.0$\% HM and $+0.3$\% HM respectively), \ours\ outperforms it on 20-2 and 20-3 ($+0.5$\% and $+1.3$\% HM). % respectively). 

Finally, we report the results for COCO-MS on tables \ref{tab:coco-ms-1} (1-shot), \ref{tab:coco-ms-2} (2-shot), and \ref{tab:coco-ms-5} (5-shot). Also in this setting \ours\ is always the best or second best method across all shots and folds. In particular, it is the best on 1-shot on every fold, outperforming the second best method (DWI) by 1.3\% HM on average.
On the 2-shot setting, \ours\ is the best on 20-0 ($+1.8$\% HM \wrt SPN) and 20-1 ($+1.2$\% HM \wrt RT) folds, being second best on 20-2 ($-1.2$\% HM \wrt SPN) and 20-3 ($-0.8$\% HM \wrt SPN). Overall, \ours\ outperforms the second best method, SPN, by $0.6$\% HM.
In the 5-shot setting, the performance of \ours\ and SPN are on par, achieving very similar results for both old and new classes. In particular, comparing them on the different folds, we see that they maintain very close performances, \ie in terms of HM, $22.9$\% vs $23.3$\% on 20-0, $22.3$\% vs $21.5$\% on 20-1, $26.4$\% vs $26.5$\% on 20-2, $29.5$\% vs $29.4$\% on 20-3, respectively for \ours\  and SPN.

\subsection{Prototype learning offline performance}
An open question from our results is whether prototype learning in the base step hampers the performance of the pretrained segmentation network. Ideally, we would like the model to retain the performance of a standard semantic segmentation model when trained offline, while keeping the advantage of prototype learning for the FSL steps.  

In this section, we show that prototype learning performs on par to other learning techniques in a standard offline setting, \ie when all the classes are learned in one step. To demonstrate this, in Tab.~\ref{tab:off-results} we report the results for a linear classifier trained with cross-entropy (std), SPN \cite{xian2019spnet}, and \ours\   %prototype learning 
on the base step of COCO. 
From the results we can see that our model is competitive with both choices, achieving an average mIoU of 52.1\% vs 53.0\% of SPN and 52.9\% of standard training. %is  \ours\ is competitive with both choices.slightly better than standard training ($0.1$\% mIoU) and \ours\  ($0.9$\% mIoU). However, we can note that \ours\  is competitive with both choices.  Moreover, we 
Note that while \ours\ performs comparably to other approaches in the offline scenario, the improvement on the incremental few-shot learning settings is remarkable, as demonstrated in previous experiments.

\subsection{Additional qualitative results}
Due to space constraints, in the paper we report only the qualitative results for VOC-SS 1-shot. Here, we expand the analysis by reporting the results for other scenarios, \ie COCO-SS 1-shot, COCO-SS 2-shot and VOC-SS 2-shot. %dataset and extending the analysis also to the 2-shot scenario.

Fig.~\ref{fig:qualitative-coco} shows some qualitative results for different methods on COCO-SS 1-shot. From the figure, we can see how \ours\ better discriminates the new class \wrt other approaches. Overall, we see that WI and DWI tend to assign pixels to new classes even when they are outside the class of interest (\eg \textit{dog} second row, \textit{wc}, fourth row), while ILT and SPN may either ignore pixels of new classes (\eg \textit{surfboard} third row) or assign them to old ones (\eg \textit{elephant} first row). On the other hand, \ours\ correctly segments both old and new classes, even in images with clutter (\eg \textit{surfboard} third row), multiple instances (\eg \textit{sheep} last row) and complex boundaries (\eg \textit{dog} second row).

In Fig.~\ref{fig:qualitative-voc2} and Fig.~\ref{fig:qualitative-coco2} we show results for the VOC-SS and COCO-SS 2-shot settings. Similarly to VOC-SS 1-shot and COCO-SS 1-shot, non-finetuned methods (WI, DWI) may not discriminate new classes, %making incoherent prediction 
when they are similar to base ones, making incoherent predictions. Examples are \textit{cow} and \textit{bus} (first and second rows of \figref{fig:qualitative-voc2}) mistakenly segmented as \textit{horse} (purple) and \textit{train} (light-green) respectively,  and \textit{giraffe} (fifth row of \figref{fig:qualitative-coco2}) segmented as \textit{zebra} (blue). SPN and ILT may not properly learn to segment new classes when trained with few complex examples. For instance, both methods fail to segment \textit{motorcycle} (third row \figref{fig:qualitative-voc2}) and \textit{sofa} (\figref{fig:qualitative-coco2}, fourth row), where training images are either small and in cluttered environments (\eg \textit{motorcycle}) or mixed with other classes (\eg \textit{dogs} in \textit{sofa}). In contrast, \ours\ precisely segments new classes, discriminating them from old ones. For instance, our model correctly segments the multiple instances of \textit{motorcycle} and \textit{sheep} (last row) in \figref{fig:qualitative-voc2}, while separating pixels of \textit{cat} and \textit{dog} from the new class \textit{sofa} in \figref{fig:qualitative-coco2}. Interestingly, \ours\ can correctly discriminate almost all pixels of the new classes (\eg \textit{cow}, second row of \figref{fig:qualitative-voc2}, \textit{bear} and {\textit{sandwich}} in \figref{fig:qualitative-coco2} second and third rows), despite their similarities (\eg \textit{cow} with \textit{horse}) or large difference (\eg \textit{bear}) with old ones, or the presence of multiple other classes (\eg \textit{sandwich}).

\begin{table}[t]
    \centering
    \begin{tabular}{l|c||c|c|c|c}
         Method  &  Mean  &  20-0  &  20-1  &  20-2  &  20-3 \\ \hline
         std  &           52.9 & 			\textbf{49.8} & 			52.6 & 			\textbf{55.1} & 			54.2 \\
         SPN \cite{xian2019spnet}   &      \textbf{53.0} & 			49.5 & 			\textbf{53.2} & 			54.7 & 			\textbf{54.6} \\
         \ours             &  52.1 & 			47.9 & 			51.6 & 			54.4 & 			54.3 \\
    \end{tabular}
    \vspace{4pt}
    \caption{mIoU on base classes, before the few-shot steps, comparing the Prototype Learning (\ours) with a standard classifier (std) and SPN \cite{xian2019spnet} on the COCO dataset.} \label{tab:off-results}
\end{table}

\begin{table*}[t]
    \centering
    \setlength{\tabcolsep}{3pt} % Default value: 6pt
    \resizebox{\linewidth}{!}
    {\begin{tabular}{ll|ccc||ccc|ccc|ccc|ccc}
     &    &   \multicolumn{3}{c||}{\textbf{Mean}}  &  \multicolumn{3}{c|}{\textbf{5-0}}  &  \multicolumn{3}{c|}{\textbf{5-1}}  &  \multicolumn{3}{c|}{\textbf{5-2}}  &  \multicolumn{3}{c}{\textbf{5-3}} \\ \hline
 &  Method	                          &  mIoU-B  &  mIoU-N	  &  HM	  &  mIoU-B  &  mIoU-N	  &  HM  &  mIoU-B  &  mIoU-N	  &  HM   &  mIoU-B  &  mIoU-N	  &  HM  &  mIoU-B  &  mIoU-N	  &  HM	  \\ \hline
 &  FT                                  &  58.3 & 9.7 & 16.7 & 61.9 & 3.2 & 6.1 & 55.2 & 16.3 & 25.2 & 53.6 & 13.1 & 21.1 & 62.4 & 6.3 & 11.5 \\ \hline
 \parbox[t]{2mm}{\multirow{3}{*}{\rotatebox[origin=c]{90}{FSC}}}
 &  WI \cite{qi2018low}                 &  62.7 & 15.5 & 24.8 & 66.5 & 10.5 & 18.1 & 58.9 & 21.9 & 31.9 & 58.6 & 15.3 & 24.2 & 66.7 & 14.2 & 23.5 \\
 &  DWI \cite{gidaris2018dynamic}       &  64.3 & 15.4 & 24.8 & 67.3 & 10.3 & 17.9 & 59.9 & 23.3 & \underline{33.5} & 60.0 & 16.0 & 25.3 & 69.9 & 11.8 & 20.2 \\
 &  RT \cite{tian2020rethinking}        &  59.1 & 12.1 & 20.1 & 62.7 & 3.8 & 7.1 & 54.5 & 18.7 & 27.9 & 56.3 & 14.6 & 23.2 & 63.1 & 11.4 & 19.3 \\ \hline
 \parbox[t]{2mm}{\multirow{2}{*}{\rotatebox[origin=c]{90}{FSS}}}
 &  AMP  \cite{siam2019adaptive}        &  57.5 & 16.7 & \underline{25.8} & 61.7 & 12.0 & \underline{20.1} & 49.8 & 22.9 & 31.4 & 54.8 & 15.3 & 23.9 & 63.5 & 16.5 & \textbf{26.1} \\
 &  SPN  \cite{xian2019spnet}           &  59.8 & 16.3 & 25.6 & 64.1 & 9.0 & 15.8 & 56.2 & 23.9 & \underline{33.5} & 56.2 & 19.3 &\underline{ 28.7} & 62.7 & 13.1 & 21.7 \\ \hline
 \parbox[t]{2mm}{\multirow{3}{*}{\rotatebox[origin=c]{90}{IL}}}
 &  LwF  \cite{li2017learning}          &  61.5 & 10.7 & 18.2 & 63.7 & 2.8 & 5.3 & 59.0 & 19.3 & 29.0 & 59.1 & 14.1 & 22.8 & 64.0 & 6.6 & 11.9 \\
 &  ILT  \cite{michieli2019incremental} &  64.3 & 13.6 & 22.5 & 67.1 & 5.9 & 10.8 & 60.5 & 19.3 & 29.2 & 61.2 & 18.9 & 28.9 & 68.4 & 10.3 & 18.0 \\
 &  MiB  \cite{cermelli2020modeling}    &  61.0 & 5.2 & 9.7 & 64.6 & 3.1 & 6.0 & 56.9 & 7.6 & 13.4 & 57.3 & 6.3 & 11.4 & 65.4 & 3.9 & 7.4 \\ \hline
 &  \textbf{\ours}                      &  60.9 & 18.6 & \textbf{28.4} & 64.4 & 12.7 & \textbf{21.2} & 54.3 & 25.1 & \textbf{34.3} & 57.1 & 20.3 & \textbf{29.9} & 67.6 & 16.2 & \textbf{26.1} \\  

    \end{tabular}}
    \vspace{-4pt} \caption{\SET: VOC-SS 1-shot.} \label{tab:voc-ss-1}
    \vspace{-4pt}
\end{table*}

\begin{table*}[t]
    \centering
    \setlength{\tabcolsep}{3pt} % Default value: 6pt
    \resizebox{\linewidth}{!}
    {\begin{tabular}{ll|ccc||ccc|ccc|ccc|ccc}
     &    &   \multicolumn{3}{c||}{\textbf{Mean}}  &  \multicolumn{3}{c|}{\textbf{5-0}}  &  \multicolumn{3}{c|}{\textbf{5-1}}  &  \multicolumn{3}{c|}{\textbf{5-2}}  &  \multicolumn{3}{c}{\textbf{5-3}} \\ \hline
 &  Method	                          &  mIoU-B  &  mIoU-N	  &  HM	  &  mIoU-B  &  mIoU-N	  &  HM  &  mIoU-B  &  mIoU-N	  &  HM   &  mIoU-B  &  mIoU-N	  &  HM  &  mIoU-B  &  mIoU-N	  &  HM	  \\ \hline
 &  FT                                  &  59.1 & 	19.7 & 	29.5 & 	61.7 & 	12.6 & 	20.9 & 	57.5 & 	31.0 & 	40.3 & 	54.8 & 	20.2 & 	29.5 & 	62.5 & 	15.0 & 	24.2 \\ \hline
\parbox[t]{2mm}{\multirow{3}{*}{\rotatebox[origin=c]{90}{FSC}}}
 &  WI \cite{qi2018low}                 &  63.3 & 	19.2 & 	29.5 & 	67.1 & 	13.1 & 	21.9 & 	59.0 & 	28.2 & 	38.2 & 	59.3 & 	18.1 & 	27.7 & 	67.7 & 	17.5 & 	27.8 \\
 &  DWI \cite{gidaris2018dynamic}       &  64.8 & 	19.8 & 	30.4 & 	68.2 & 	15.1 & 	24.7 & 	60.4 & 	30.9 & 	40.9 & 	60.4 & 	17.2 & 	26.8 & 	70.1 & 	16.2 & 	26.3 \\
 &  RT \cite{tian2020rethinking}        &  60.9 & 	21.6 & 	31.9 & 	65.3 & 	10.4 & 	18.0 & 	54.4 & 	34.6 & 	42.3 & 	59.2 & 	24.3 & 	34.5 & 	64.7 & 	17.0 & 	27.0 \\ \hline
\parbox[t]{2mm}{\multirow{2}{*}{\rotatebox[origin=c]{90}{FSS}}}
 &  AMP  \cite{siam2019adaptive}        &  54.4 & 	18.8 & 	27.9 & 	59.7 & 	12.5 & 	20.7 & 	44.5 & 	28.4 & 	34.7 & 	53.4 & 	17.2 & 	26.0 & 	59.8 & 	17.0 & 	26.5 \\
 &  SPN  \cite{xian2019spnet}           &  60.8 & 	26.3 & 	\underline{36.7 }& 	65.5 & 	18.8 & \textbf{	29.2} & 	57.1 & 	37.4 & 	\textbf{45.2} & 	57.8 & 	25.6 & \underline{	35.5} & 	62.7 & 	23.4 & 	\underline{34.1} \\ \hline
\parbox[t]{2mm}{\multirow{3}{*}{\rotatebox[origin=c]{90}{IL}}}
 &  LwF  \cite{li2017learning}          &  63.6 & 	18.9 & 	29.2 & 	65.2 & 	10.8 & 	18.6 & 	61.8 & 	31.3 & 	41.6 & 	60.9 & 	21.0 & 	31.3 & 	66.5 & 	12.6 & 	21.2 \\
 &  ILT  \cite{michieli2019incremental} &  64.2 & 	23.1 & 	34.0 & 	68.4 & 	16.1 & 	26.1 & 	58.3 & 	33.7 & 	42.7 & 	61.1 & 	25.6 & 	36.1 & 	68.9 & 	17.1 & 	27.4 \\
 &  MiB  \cite{cermelli2020modeling}    &  63.5 & 	12.7 & 	21.1 & 	66.6 & 	12.3 & 	20.7 & 	60.1 & 	18.3 & 	28.0 & 	59.7 & 	11.2 & 	18.8 & 	67.7 & 	9.0 & 	15.8 \\ \hline
 &  \textbf{\ours}                      &  60.5 & 	26.4 & 	\textbf{36.8} & 	64.0 & 	18.9 & 	\underline{29.1} & 	53.9 & 	36.6 & 	\underline{43.6} & 	58.2 & 	26.5 & 	\textbf{36.4} & 	65.9 & 	23.6 & \textbf{	34.7} \\  

    \end{tabular}}
    \vspace{-4pt} \caption{\SET: VOC-SS 2-shot.} \label{tab:voc-ss-2}
    \vspace{-4pt}
\end{table*}

\begin{table*}[t]
    \centering
    \setlength{\tabcolsep}{3pt} % Default value: 6pt
    \resizebox{\linewidth}{!}
    {\begin{tabular}{ll|ccc||ccc|ccc|ccc|ccc}
     &    &   \multicolumn{3}{c||}{\textbf{Mean}}  &  \multicolumn{3}{c|}{\textbf{5-0}}  &  \multicolumn{3}{c|}{\textbf{5-1}}  &  \multicolumn{3}{c|}{\textbf{5-2}}  &  \multicolumn{3}{c}{\textbf{5-3}} \\ \hline
 &  Method	                          &  mIoU-B  &  mIoU-N	  &  HM	  &  mIoU-B  &  mIoU-N	  &  HM  &  mIoU-B  &  mIoU-N	  &  HM   &  mIoU-B  &  mIoU-N	  &  HM  &  mIoU-B  &  mIoU-N	  &  HM	  \\ \hline
 &  FT                                  &  55.8 & 	29.6 & 	38.7 & 	58.4 & 	22.8 & 	32.8 & 	52.3 & 	42.7 & 	47.0 & 	50.6 & 	29.7 & 	37.5 & 	62.0 & 	23.0 & 	33.6 \\ \hline
\parbox[t]{2mm}{\multirow{3}{*}{\rotatebox[origin=c]{90}{FSC}}}
 &  WI \cite{qi2018low}                 &  63.3 & 	21.7 & 	32.3 & 	67.5 & 	16.3 & 	26.3 & 	58.7 & 	30.8 & 	40.4 & 	59.4 & 	21.3 & 	31.4 & 	67.5 & 	18.4 & 	28.9 \\
 &  DWI \cite{gidaris2018dynamic}       &  64.9 & 	23.5 & 	34.5 & 	68.8 & 	20.7 & 	31.8 & 	60.8 & 	34.7 & 	44.2 & 	60.9 & 	20.6 & 	30.7 & 	69.1 & 	17.9 & 	28.5 \\
 &  RT \cite{tian2020rethinking}        &  60.4 & 	27.5 & 	37.8 & 	65.6 & 	19.1 & 	29.6 & 	55.8 & 	38.8 & 	45.8 & 	55.1 & 	29.3 & 	38.3 & 	65.0 & 	22.9 & 	33.9 \\ \hline
 \parbox[t]{2mm}{\multirow{2}{*}{\rotatebox[origin=c]{90}{FSS}}}
 &  AMP  \cite{siam2019adaptive}        &  51.9 & 	18.9 & 	27.7 & 	58.5 & 	12.9 & 	21.2 & 	38.5 & 	26.5 & 	31.4 & 	51.9 & 	20.4 & 	29.3 & 	58.5 & 	15.8 & 	24.8 \\
 &  SPN  \cite{xian2019spnet}           &  58.4 & 	33.4 & 	\underline{42.5} & 	63.3 & 	28.2 & 	\underline{39.0 }& 	53.4 & 	43.7 & 	\underline{48.1} & 	54.5 & 	33.5 & 	41.5 & 	62.3 & 	28.2 & 	\underline{38.8} \\ \hline
\parbox[t]{2mm}{\multirow{3}{*}{\rotatebox[origin=c]{90}{IL}}}
 &  LwF  \cite{li2017learning}          &  59.7 & 	30.9 & 	40.8 & 	62.8 & 	23.9 & 	34.6 & 	57.1 & 	44.0 & 	\textbf{49.7} & 	55.9 & 	31.6 & 	40.3 & 	63.0 & 	24.4 & 	35.2 \\
 &  ILT  \cite{michieli2019incremental} &  61.4 & 	32.0 & 	42.1 & 	67.2 & 	27.8 & 	\textbf{39.4} & 	54.2 & 	40.4 & 	46.3 & 	57.1 & 	33.8 & 	\underline{42.4} & 	67.0 & 	26.1 & 	37.5 \\
 &  MiB  \cite{cermelli2020modeling}    &  65.0 & 	28.1 & 	39.3 & 	68.0 & 	24.8 & 	36.4 & 	62.1 & 	35.2 & 	44.9 & 	60.6 & 	27.1 & 	37.4 & 	69.1 & 	25.4 & 	37.2 \\ \hline
 &  \textbf{\ours}                      &  60.0 & 	33.3 & 	\textbf{42.8 }& 	64.3 & 	26.7 & 	37.7 & 	53.3 & 	41.0 & 	46.3 & 	57.4 & 	33.8 & \textbf{	42.5} & 	65.2 & 	31.6 & \textbf{42.6} \\  

    \end{tabular}}
    \vspace{-4pt} \caption{\SET: VOC-SS 5-shot.} \label{tab:voc-ss-5}
    \vspace{-4pt}
\end{table*}

\begin{table*}[t]
    \centering
    \setlength{\tabcolsep}{3pt} % Default value: 6pt
    \resizebox{\linewidth}{!}
    {\begin{tabular}{ll|ccc||ccc|ccc|ccc|ccc}
     &    &   \multicolumn{3}{c||}{\textbf{Mean}}  &  \multicolumn{3}{c|}{\textbf{5-0}}  &  \multicolumn{3}{c|}{\textbf{5-1}}  &  \multicolumn{3}{c|}{\textbf{5-2}}  &  \multicolumn{3}{c}{\textbf{5-3}} \\ \hline
 &  Method	                          &  mIoU-B  &  mIoU-N	  &  HM	  &  mIoU-B  &  mIoU-N	  &  HM  &  mIoU-B  &  mIoU-N	  &  HM   &  mIoU-B  &  mIoU-N	  &  HM  &  mIoU-B  &  mIoU-N	  &  HM	  \\ \hline
 &  FT                                  &  47.2 & 	3.9 & 	7.2 & 	46.8 & 	2.0 & 	3.8 & 	42.0 & 	8.0 & 	13.4 & 	47.3 & 	3.5 & 	6.5 & 	52.7 & 	2.1 & 	4.0 \\ \hline
\parbox[t]{2mm}{\multirow{3}{*}{\rotatebox[origin=c]{90}{FSC}}}
 &  WI \cite{qi2018low}                 &  66.6 & 	16.1 & 	25.9 & 	68.8 & 	14.9 & 	\underline{24.5} & 	63.5 & 	24.4 & 	35.3 & 	63.3 & 	14.3 & 	\underline{23.4} & 	70.9 & 	10.6 & 	18.5 \\
 &  DWI \cite{gidaris2018dynamic}       &  67.2 & 	16.3 & \underline{26.2} & 69.0 & 15.7 & \textbf{25.6} & 63.6 & 25.8 & \underline{36.7} & 64.1 & 13.6 & 22.5 & 71.9 & 10.0 & 17.6 \\
 &  RT \cite{tian2020rethinking}        &  49.2 & 5.8 & 10.4 & 45.4 & 2.2 & 4.2 & 41.5 & 12.4 & 19.1 & 46.7 & 4.8 & 8.6 & 53.3 & 4.5 & 8.2 \\ \hline
\parbox[t]{2mm}{\multirow{2}{*}{\rotatebox[origin=c]{90}{FSS}}}
 &  AMP  \cite{siam2019adaptive}        &  58.6 & 14.5 & 23.2 & 61.6 & 12.1 & 20.2 & 54.5 & 22.8 & 32.1 & 56.1 & 11.8 & 19.5 & 62.4 & 11.3 &\underline{ 19.1} \\
 &  SPN  \cite{xian2019spnet}           &  49.8 & 8.1 & 13.9 & 48.7 & 3.6 & 6.6 & 44.0 & 13.7 & 20.9 & 51.4 & 8.7 & 14.9 & 55.0 & 6.5 & 11.7 \\ \hline
\parbox[t]{2mm}{\multirow{3}{*}{\rotatebox[origin=c]{90}{IL}}}
 &  LwF  \cite{li2017learning}          &  42.1 & 3.3 & 6.2 & 42.1 & 1.8 & 3.4 & 37.9 & 6.8 & 11.5 & 41.4 & 2.5 & 4.7 & 47.1 & 2.2 & 4.3 \\
 &  ILT  \cite{michieli2019incremental} &  43.7 & 3.3 & 6.1 & 42.3 & 1.7 & 3.3 & 41.0 & 6.1 & 10.6 & 41.9 & 3.5 & 6.4 & 49.6 & 1.8 & 3.4 \\
 &  MiB  \cite{cermelli2020modeling}    &  43.9 & 2.6 & 4.9 & 41.0 & 1.0 & 2.0 & 40.2 & 5.8 & 10.2 & 43.4 & 2.4 & 4.5 & 51.0 & 1.1 & 2.2 \\ \hline
 &  \textbf{\ours}                      &  64.1 & 	16.9 & 	\textbf{26.7} & 	67.6 & 	13.3 & 	22.3 & 	58.0 & 	27.1 & 	\textbf{36.9} & 	61.0 & 	15.6 & 	\textbf{24.9} & 	69.8 & 	11.5 & 	\textbf{19.8} \\  

    \end{tabular}}
    \vspace{-4pt} \caption{\SET: VOC-MS 1-shot.} \label{tab:voc-ms-1}
    \vspace{-4pt}
\end{table*}

\begin{table*}[t]
    \centering
    \setlength{\tabcolsep}{3pt} % Default value: 6pt
    \resizebox{\linewidth}{!}
    {\begin{tabular}{ll|ccc||ccc|ccc|ccc|ccc}
     &    &   \multicolumn{3}{c||}{\textbf{Mean}}  &  \multicolumn{3}{c|}{\textbf{5-0}}  &  \multicolumn{3}{c|}{\textbf{5-1}}  &  \multicolumn{3}{c|}{\textbf{5-2}}  &  \multicolumn{3}{c}{\textbf{5-3}} \\ \hline
 &  Method	                          &  mIoU-B  &  mIoU-N	  &  HM	  &  mIoU-B  &  mIoU-N	  &  HM  &  mIoU-B  &  mIoU-N	  &  HM   &  mIoU-B  &  mIoU-N	  &  HM  &  mIoU-B  &  mIoU-N	  &  HM	  \\ \hline
 &  FT                                  &  53.5 & 4.4 & 8.1 & 54.5 & 2.3 & 4.5 & 51.2 & 8.9 & 15.2 & 51.5 & 4.3 & 7.9 & 56.9 & 2.2 & 4.3 \\ \hline
\parbox[t]{2mm}{\multirow{3}{*}{\rotatebox[origin=c]{90}{FSC}}}
 &  WI \cite{qi2018low}                 &  66.6 & 19.8 & 30.5 & 69.1 & 17.1 & 27.4 & 63.7 & 31.9 & 42.5 & 63.5 & 16.7 & \underline{26.5} & 70.3 & 13.5 & 22.7 \\
 &  DWI \cite{gidaris2018dynamic}       &  67.5 & 21.6 & \underline{32.7} & 69.7 & 21.3 & \textbf{32.6} & 63.9 & 35.4 & \underline{45.6} & 64.3 & 15.8 & 25.4 & 72.0 & 14.0 & \underline{23.5} \\
 &  RT \cite{tian2020rethinking}        &  36.0 & 4.9 & 8.6 & 43.8 & 3.1 & 5.8 & 23.0 & 7.2 & 11.0 & 28.3 & 5.3 & 9.0 & 40.7 & 4.7 & 8.5 \\ \hline
\parbox[t]{2mm}{\multirow{2}{*}{\rotatebox[origin=c]{90}{FSS}}}
 &  AMP  \cite{siam2019adaptive}        &  58.4 & 16.3 & 25.5 & 62.3 & 12.3 & 20.6 & 54.0 & 27.2 & 36.1 & 55.9 & 14.7 & 23.3 & 61.5 & 10.8 & 18.4 \\
 &  SPN  \cite{xian2019spnet}           &  56.4 & 10.4 & 17.6 & 58.3 & 5.8 & 10.6 & 54.0 & 18.2 & 27.2 & 55.6 & 10.4 & 17.5 & 57.8 & 7.3 & 13.0 \\ \hline
\parbox[t]{2mm}{\multirow{3}{*}{\rotatebox[origin=c]{90}{IL}}}
 &  LwF  \cite{li2017learning}          &  51.6 & 3.9 & 7.3 & 50.7 & 1.9 & 3.7 & 49.4 & 8.6 & 14.7 & 50.4 & 3.4 & 6.3 & 55.9 & 1.7 & 3.4 \\
 &  ILT  \cite{michieli2019incremental} &  52.2 & 4.4 & 8.1 & 50.7 & 2.0 & 3.9 & 51.6 & 9.7 & 16.3 & 49.9 & 4.0 & 7.4 & 56.8 & 1.7 & 3.4 \\
 &  MiB  \cite{cermelli2020modeling}    &  51.9 & 2.1 & 4.0 & 52.7 & 1.7 & 3.4 & 47.9 & 3.4 & 6.4 & 50.6 & 2.5 & 4.7 & 56.4 & 0.8 & 1.5 \\ \hline
 &  \textbf{\ours}                      &  65.2 & 23.7 & \textbf{34.8} & 68.0 & 17.7 & \underline{28.1} & 61.3 & 40.4 & \textbf{48.7} & 62.5 & 21.8 & \textbf{32.4} & 69.2 & 15.0 & \textbf{24.7} \\  

    \end{tabular}}
    \vspace{-4pt} \caption{\SET: VOC-MS 2-shot.} \label{tab:voc-ms-2}
    \vspace{-4pt}
\end{table*}

\begin{table*}[t]
    \centering
    \setlength{\tabcolsep}{3pt} % Default value: 6pt
    \resizebox{\linewidth}{!}
    {\begin{tabular}{ll|ccc||ccc|ccc|ccc|ccc}
     &    &   \multicolumn{3}{c||}{\textbf{Mean}}  &  \multicolumn{3}{c|}{\textbf{5-0}}  &  \multicolumn{3}{c|}{\textbf{5-1}}  &  \multicolumn{3}{c|}{\textbf{5-2}}  &  \multicolumn{3}{c}{\textbf{5-3}} \\ \hline
 &  Method	                          &  mIoU-B  &  mIoU-N	  &  HM	  &  mIoU-B  &  mIoU-N	  &  HM  &  mIoU-B  &  mIoU-N	  &  HM   &  mIoU-B  &  mIoU-N	  &  HM  &  mIoU-B  &  mIoU-N	  &  HM	  \\ \hline
 &  FT                                  &  58.7 & 7.7 & 13.6 & 59.9 & 5.1 & 9.5 & 57.0 & 14.8 & 23.5 & 55.9 & 7.1 & 12.5 & 62.5 & 3.7 & 7.0 \\ \hline
\parbox[t]{2mm}{\multirow{3}{*}{\rotatebox[origin=c]{90}{FSC}}}
 &  WI \cite{qi2018low}                 &  66.6 & 21.9 & 33.0 & 69.6 & 20.4 & 31.5 & 63.4 & 32.9 & 43.3 & 63.4 & 20.1 & \underline{30.6} & 69.9 & 14.3 & 23.8 \\
 &  DWI \cite{gidaris2018dynamic}       &  67.6 & 25.4 & \underline{36.9} & 70.3 & 27.9 & \textbf{39.9} & 64.1 & 38.0 & \underline{47.7} & 64.5 & 19.6 & 30.1 & 71.5 & 16.0 & \underline{26.1} \\
 &  RT \cite{tian2020rethinking}        &  45.1 & 10.0 & 16.4  & 52.5 & 7.3 & 12.7 & 35.4 & 16.7 & 22.7 & 39.4 & 9.3 & 15.0 & 53.1 & 6.9 & 12.2 \\ \hline
\parbox[t]{2mm}{\multirow{2}{*}{\rotatebox[origin=c]{90}{FSS}}}
 &  AMP  \cite{siam2019adaptive}        &  57.1 & 17.2 & 26.4 & 62.5 & 13.5 & 22.2 & 50.1 & 25.3 & 33.7 & 55.1 & 18.7 & 28.0 & 60.8 & 11.2 & 18.9 \\
 &  SPN  \cite{xian2019spnet}           &  61.6 & 16.3 & 25.8 & 62.3 & 10.4 & 17.9 & 59.5 & 27.6 & 37.7 & 60.3 & 14.7 & 23.7 & 64.2 & 12.3 & 20.6 \\ \hline
\parbox[t]{2mm}{\multirow{3}{*}{\rotatebox[origin=c]{90}{IL}}}
 &  LwF  \cite{li2017learning}          &  59.8 & 7.5 & 13.4 & 60.7 & 5.2 & 9.6 & 57.8 & 14.6 & 23.3 & 57.4 & 6.8 & 12.2 & 63.3 & 3.5 & 6.6 \\
 &  ILT  \cite{michieli2019incremental} &  59.0 & 7.9 & 13.9 & 59.9 & 5.4 & 9.8 & 57.0 & 15.0 & 23.8 & 56.0 & 7.1 & 12.6 & 62.9 & 4.0 & 7.6 \\
 &  MiB  \cite{cermelli2020modeling}    &  60.9 & 5.8 & 10.5 & 61.0 & 4.8 & 8.9 & 58.4 & 9.6 & 16.5 & 59.5 & 5.9 & 10.8 & 64.9 & 2.7 & 5.2 \\ \hline
 &  \textbf{\ours}                      &  64.5 & 27.5 & \textbf{38.6} & 67.4 & 23.8 & \underline{35.2} & 60.4 & 41.6 & \textbf{49.3} & 61.6 & 25.4 & \textbf{35.9} & 68.6 & 19.0 &\textbf{ 29.8} \\  

    \end{tabular}}
    \vspace{-4pt} \caption{\SET: VOC-MS 5-shot.} \label{tab:voc-ms-5}
    \vspace{-4pt}
\end{table*}

\begin{table*}[t]
    \centering
    \setlength{\tabcolsep}{3pt} % Default value: 6pt
    \resizebox{\linewidth}{!}
    {\begin{tabular}{ll|ccc||ccc|ccc|ccc|ccc}
     &    &   \multicolumn{3}{c||}{\textbf{Mean}}  &  \multicolumn{3}{c|}{\textbf{20-0}}  &  \multicolumn{3}{c|}{\textbf{20-1}}  &  \multicolumn{3}{c|}{\textbf{20-2}}  &  \multicolumn{3}{c}{\textbf{20-3}} \\ \hline
 &  Method	                          &  mIoU-B  &  mIoU-N	  &  HM	  &  mIoU-B  &  mIoU-N	  &  HM  &  mIoU-B  &  mIoU-N	  &  HM   &  mIoU-B  &  mIoU-N	  &  HM  &  mIoU-B  &  mIoU-N	  &  HM	  \\ \hline
 &  FT                                  &  41.2 & 4.1 & 7.5 & 36.2 & 2.0 & 3.8 & 40.6 & 4.9 & 8.7 & 45.0 & 3.7 & 6.8 & 43.1 & 5.8 & 10.3 \\ \hline
\parbox[t]{2mm}{\multirow{3}{*}{\rotatebox[origin=c]{90}{FSC}}}
 &  WI \cite{qi2018low}                 &  43.8 & 6.9 & 11.9 & 41.0 & 4.8 & 8.6 & 42.8 & 7.8 & 13.2 & 46.4 & 6.8 & 11.8 & 45.1 & 8.1 & 13.8 \\
 &  DWI \cite{gidaris2018dynamic}       &  44.5 & 7.5 & \underline{12.8} & 39.8 & 5.0 & \underline{8.9} & 44.4 & 8.2 & \underline{13.9} & 47.2 & 6.8 & 11.9 & 46.6 & 9.9 & \underline{16.4} \\
 &  RT \cite{tian2020rethinking}        &  46.2 & 5.8 & 10.2 & 39.4 & 3.4 & 6.2 & 46.5 & 6.1 & 10.8 & 50.4 & 5.3 & 9.6 & 48.4 & 8.2 & 14.1 \\ \hline
\parbox[t]{2mm}{\multirow{2}{*}{\rotatebox[origin=c]{90}{FSS}}}
 &  AMP  \cite{siam2019adaptive}        &  37.5 & 7.4 & 12.4 & 33.4 & 4.8 & 8.4 & 37.4 & 8.4 & 13.8 & 39.9 & 8.7 & \textbf{14.2} & 39.1 & 7.8 & 13.0 \\
 &  SPN  \cite{xian2019spnet}           &  43.5 & 6.7 & 11.7 & 39.2 & 4.6 & 8.2 & 43.7 & 6.4 & 11.1 & 46.8 & 7.1 & 12.3 & 44.3 & 8.9 & 14.8 \\ \hline
\parbox[t]{2mm}{\multirow{3}{*}{\rotatebox[origin=c]{90}{IL}}}
 &  LwF  \cite{li2017learning}          &  43.9 & 3.8 & 7.0 & 37.8 & 1.8 & 3.4 & 43.7 & 4.3 & 7.9 & 47.9 & 3.7 & 6.8 & 46.1 & 5.4 &  9.6 \\
 &  ILT  \cite{michieli2019incremental} &  46.2 & 4.4 & 8.0 & 40.7 & 2.4 & 4.5 & 46.0 & 4.4 & 8.1 & 50.3 & 4.7 & 8.6 & 47.8 & 6.0 & 10.6 \\
 &  MiB  \cite{cermelli2020modeling}    &  43.8 & 3.5 & 6.5 & 37.5 & 2.1 & 4.0 & 44.1 & 3.6 & 6.6 & 47.6 & 3.9 & 7.1 & 46.0 & 4.4 &  8.1  \\ \hline
 &  \textbf{\ours}                      &  40.8 & 8.2 & \textbf{13.6} & 38.6 & 5.4 & \textbf{9.5} & 39.7 & 8.6 & \textbf{14.2} & 43.5 & 7.7 & \underline{13.1} & 41.4 & 10.9 & \textbf{17.2} \\  

    \end{tabular}}
    \vspace{-4pt} \caption{\SET: COCO-SS 1-shot.} \label{tab:coco-ss-1}
    \vspace{-4pt}
\end{table*}

\begin{table*}[t]
    \centering
    \setlength{\tabcolsep}{3pt} % Default value: 6pt
    \resizebox{\linewidth}{!}
    {\begin{tabular}{ll|ccc||ccc|ccc|ccc|ccc}
     &    &   \multicolumn{3}{c||}{\textbf{Mean}}  &  \multicolumn{3}{c|}{\textbf{20-0}}  &  \multicolumn{3}{c|}{\textbf{20-1}}  &  \multicolumn{3}{c|}{\textbf{20-2}}  &  \multicolumn{3}{c}{\textbf{20-3}} \\ \hline
 &  Method	                          &  mIoU-B  &  mIoU-N	  &  HM	  &  mIoU-B  &  mIoU-N	  &  HM  &  mIoU-B  &  mIoU-N	  &  HM   &  mIoU-B  &  mIoU-N	  &  HM  &  mIoU-B  &  mIoU-N	  &  HM	  \\ \hline
 &  FT                                  &  41.5 & 7.3 & 12.4 & 37.4 & 4.2 & 7.6 & 40.3 & 9.0 & 14.7 & 45.4 & 7.7 & 13.2 & 43.1 & 8.4 & 14.0 \\ \hline
\parbox[t]{2mm}{\multirow{3}{*}{\rotatebox[origin=c]{90}{FSC}}}
 &  WI \cite{qi2018low}                 &  44.2 & 7.9 & 13.5 & 41.8 & 5.2 & 9.2 & 43.3 & 9.8 & 16.0 & 46.8 & 7.6 & 13.1 & 44.7 & 9.2 & 15.3 \\
 &  DWI \cite{gidaris2018dynamic}       &  45.0 & 9.4 & 15.6 & 40.4 & 6.1 & 10.6 & 45.2 & 10.7 & 17.4 & 47.4 & 9.1 & 15.3 & 46.9 & 11.8 & \underline{18.8} \\
 &  RT \cite{tian2020rethinking}        &  46.7 & 8.8 & 14.8 & 40.6 & 5.5 & 9.7 & 46.8 & 10.5 & 17.2 & 50.8 & 8.1 & 14.0 & 48.5 & 11.1 & 18.1 \\ \hline
\parbox[t]{2mm}{\multirow{2}{*}{\rotatebox[origin=c]{90}{FSS}}}
 &  AMP  \cite{siam2019adaptive}        &  35.7 & 8.8 & 14.2 & 30.9 & 5.8 & 9.8 & 36.2 & 10.5 & 16.3 & 38.4 & 9.2 & 14.8 & 37.3 & 9.9 & 15.6 \\
 &  SPN  \cite{xian2019spnet}           &  43.7 & 10.2 & \underline{16.5} & 40.0 & 6.7 & \underline{11.5} & 43.3 & 11.5 & \underline{18.1} & 47.0 & 10.7 & \underline{17.5} & 44.6 & 11.9 & 18.7 \\ \hline
\parbox[t]{2mm}{\multirow{3}{*}{\rotatebox[origin=c]{90}{IL}}}
 &  LwF  \cite{li2017learning}          &  44.3 & 7.1 & 12.3 & 39.2 & 4.5 & 8.0 & 43.8 & 8.7 & 14.5 & 48.1 & 7.3 & 12.7 & 46.0 & 8.0 & 13.6 \\
 &  ILT  \cite{michieli2019incremental} &  46.3 & 6.5 & 11.5 & 40.5 & 4.5 & 8.1 & 46.3 & 7.1 & 12.3 & 50.4 & 6.7 & 11.8 & 48.1 & 7.9 & 13.5 \\
 &  MiB  \cite{cermelli2020modeling}    &  44.4 & 6.0 & 10.6 & 38.2 & 4.2 & 7.6 & 44.5 & 7.1 & 12.3 & 48.6 & 6.5 & 11.4 & 46.3 & 6.1 & 10.8 \\ \hline
 &  \textbf{\ours}                      &  40.9 & 11.1 & \textbf{17.5} & 38.6 & 6.8 & \textbf{11.6} & 39.4 & 13.1 & \textbf{19.7} & 43.5 & 11.4 &\textbf{ 18.1} & 42.2 & 13.1 &\textbf{ 20.0} \\  

    \end{tabular}}
    \vspace{-4pt} \caption{\SET: COCO-SS 2-shot.} \label{tab:coco-ss-2}
    \vspace{-4pt}
\end{table*}

\begin{table*}[t]
    \centering
    \setlength{\tabcolsep}{3pt} % Default value: 6pt
    \resizebox{\linewidth}{!}
    {\begin{tabular}{ll|ccc||ccc|ccc|ccc|ccc}
     &    &   \multicolumn{3}{c||}{\textbf{Mean}}  &  \multicolumn{3}{c|}{\textbf{20-0}}  &  \multicolumn{3}{c|}{\textbf{20-1}}  &  \multicolumn{3}{c|}{\textbf{20-2}}  &  \multicolumn{3}{c}{\textbf{20-3}} \\ \hline
 &  Method	                          &  mIoU-B  &  mIoU-N	  &  HM	  &  mIoU-B  &  mIoU-N	  &  HM  &  mIoU-B  &  mIoU-N	  &  HM   &  mIoU-B  &  mIoU-N	  &  HM  &  mIoU-B  &  mIoU-N	  &  HM	  \\ \hline
 &  FT                                  &  41.6 & 12.3 & 19.0 & 37.3 & 7.6 & 12.6 & 40.9 & 15.0 & 22.0 & 45.3 & 13.7 & 21.0 & 43.0 & 12.9 & 19.8 \\ \hline
\parbox[t]{2mm}{\multirow{3}{*}{\rotatebox[origin=c]{90}{FSC}}}
 &  WI \cite{qi2018low}                 &  43.6 & 8.7 & 14.6 & 41.7 & 6.0 & 10.5 & 42.8 & 10.7 & 17.1 & 45.7 & 8.6 & 14.4 & 44.4 & 9.7 & 15.9 \\
 &  DWI \cite{gidaris2018dynamic}       &  44.9 & 12.1 & 19.1 & 40.5 & 8.2 & 13.6 & 45.3 & 14.4 & 21.9 & 47.0 & 12.2 & 19.4 & 46.7 & 13.7 & 21.2 \\
 &  RT \cite{tian2020rethinking}        &  46.9 & 13.7 & 21.2 & 41.1 & 9.5 & 15.4 & 46.4 & 15.9 & 23.7 & 50.7 & 13.8 & 21.6 & 49.1 & 15.7 & 23.8 \\ \hline
\parbox[t]{2mm}{\multirow{2}{*}{\rotatebox[origin=c]{90}{FSS}}}
 &  AMP  \cite{siam2019adaptive}        &  34.6 & 11.0 & 16.7 & 31.2 & 7.2 & 11.6 & 34.8 & 14.5 & 20.4 & 36.9 & 10.9 & 16.8 & 35.6 & 11.5 & 17.4 \\
 &  SPN  \cite{xian2019spnet}           &  43.7 & 15.6 & \textbf{22.9} & 40.1 & 11.5 &\textbf{ 17.9} & 42.9 & 17.7 &\textbf{ 25.1} & 46.4 & 16.4 & \underline{24.2} & 45.4 & 16.6 & \underline{24.4} \\ \hline
\parbox[t]{2mm}{\multirow{3}{*}{\rotatebox[origin=c]{90}{IL}}}
 &  LwF  \cite{li2017learning}          &  44.6 & 12.9 & 20.1 & 39.6 & 8.0 & 13.3 & 43.7 & 15.9 & 23.3 & 48.6 & 14.1 & 21.9 & 46.4 & 13.8 & 21.2 \\
 &  ILT  \cite{michieli2019incremental} &  47.0 & 11.0 & 17.8 & 41.9 & 7.1 & 12.2 & 47.0 & 13.9 & 21.5 & 50.4 & 11.2 & 18.3 & 48.6 & 11.8 & 19.0 \\
 &  MiB  \cite{cermelli2020modeling}    &  44.7 & 11.9 & 18.8 & 38.2 & 8.1 & 13.4 & 44.9 & 13.9 & 21.2 & 49.0 & 13.4 & 21.0 & 46.7 & 12.2 & 19.3 \\ \hline
 &  \textbf{\ours}                      &  42.8 & 15.7 & \textbf{23.0} & 40.6 & 10.7 & \underline{16.9} & 41.5 & 17.7 & \underline{24.8} & 45.3 & 16.9 & \textbf{24.7} & 43.9 & 17.5 & \textbf{25.0} \\  

    \end{tabular}}
    \vspace{-4pt} \caption{\SET: COCO-SS 5-shot.} \label{tab:coco-ss-5}
    \vspace{-4pt}
\end{table*}

\begin{table*}[t]
    \centering
    \setlength{\tabcolsep}{3pt} % Default value: 6pt
    \resizebox{\linewidth}{!}
    {\begin{tabular}{ll|ccc||ccc|ccc|ccc|ccc}
     &    &   \multicolumn{3}{c||}{\textbf{Mean}}  &  \multicolumn{3}{c|}{\textbf{20-0}}  &  \multicolumn{3}{c|}{\textbf{20-1}}  &  \multicolumn{3}{c|}{\textbf{20-2}}  &  \multicolumn{3}{c}{\textbf{20-3}} \\ \hline
 &  Method	                          &  mIoU-B  &  mIoU-N	  &  HM	  &  mIoU-B  &  mIoU-N	  &  HM  &  mIoU-B  &  mIoU-N	  &  HM   &  mIoU-B  &  mIoU-N	  &  HM  &  mIoU-B  &  mIoU-N	  &  HM	  \\ \hline
 &  FT                                  &  38.5 & 4.8 & 8.6 & 33.3 & 3.8 & 6.8 & 39.8 & 3.6 & 6.6 & 40.3 & 4.1 & 7.5 & 40.5 & 7.8 & 13.1 \\ \hline
\parbox[t]{2mm}{\multirow{3}{*}{\rotatebox[origin=c]{90}{FSC}}}
 &  WI \cite{qi2018low}                 &  46.3 & 8.3 & 14.0 & 42.6 & 5.6 & 9.9 & 45.9 & 9.1 & 15.2 & 48.9 & 8.1 & 13.8 & 47.9 & 10.3 & 17.0 \\
 &  DWI \cite{gidaris2018dynamic}       &  46.2 & 9.2 & \underline{15.3} & 41.0 & 5.7 & 9.9 & 46.5 & 9.7 & \textbf{16.0} & 48.8 & 8.6 &\underline{ 14.7} & 48.6 & 12.7 & \underline{20.1} \\
 &  RT \cite{tian2020rethinking}        &  38.4 & 5.2 & 9.1 & 34.4 & 2.5 & 4.6 & 42.2 & 5.7 & 10.1 & 45.1 & 6.0 & 10.6 & 31.8 & 6.4 & 10.7 \\ \hline
\parbox[t]{2mm}{\multirow{2}{*}{\rotatebox[origin=c]{90}{FSS}}}
 &  AMP  \cite{siam2019adaptive}        &  36.6 & 7.9 & 13.1 & 34.0 & 6.7 & 11.2 & 36.7 & 8.0 & 13.2 & 38.5 & 8.2 & 13.6 & 37.2 & 8.8 & 14.2 \\
 &  SPN  \cite{xian2019spnet}           &  40.3 & 8.7 & 14.3 & 37.1 & 7.5 & \underline{12.4} & 41.1 & 7.0 & 11.9 & 42.3 & 8.2 & 13.7 & 40.6 & 12.2 & 18.8 \\ \hline
\parbox[t]{2mm}{\multirow{3}{*}{\rotatebox[origin=c]{90}{IL}}}
 &  LwF  \cite{li2017learning}          &  41.0 & 4.1 & 7.4 & 35.5 & 3.3 & 6.0 & 42.4 & 2.7 & 5.2 & 42.9 & 3.8 & 6.9 & 43.1 & 6.6 & 11.4 \\
 &  ILT  \cite{michieli2019incremental} &  43.7 & 6.2 & 10.8 & 38.5 & 4.8 & 8.5 & 45.0 & 4.8 & 8.7 & 45.8 & 5.2 & 9.4 & 45.5 & 10.0 & 16.4 \\
 &  MiB  \cite{cermelli2020modeling}    &  40.4 & 3.1 & 5.8 & 32.8 & 1.2 & 2.4 & 41.5 & 2.3 & 4.4 & 43.9 & 3.9 & 7.1 & 43.4 & 5.0 & 9.0 \\ \hline
 &  \textbf{\ours}                      &  40.4 & 10.4 & \textbf{16.6} & 37.0 & 8.3 & \textbf{13.6} & 40.5 & 10.0 & \textbf{16.0 }& 42.0 & 9.1 & \textbf{15.0} & 42.3 & 14.3 & \textbf{21.4} \\  

    \end{tabular}}
    \vspace{-4pt} \caption{\SET: COCO-MS 1-shot.} \label{tab:coco-ms-1}
    \vspace{-4pt}
\end{table*}
\begin{table*}[t]
    \centering
    \setlength{\tabcolsep}{3pt} % Default value: 6pt
    \resizebox{\linewidth}{!}
    {\begin{tabular}{ll|ccc||ccc|ccc|ccc|ccc}
     &    &   \multicolumn{3}{c||}{\textbf{Mean}}  &  \multicolumn{3}{c|}{\textbf{20-0}}  &  \multicolumn{3}{c|}{\textbf{20-1}}  &  \multicolumn{3}{c|}{\textbf{20-2}}  &  \multicolumn{3}{c}{\textbf{20-3}} \\ \hline
 &  Method	                          &  mIoU-B  &  mIoU-N	  &  HM	  &  mIoU-B  &  mIoU-N	  &  HM  &  mIoU-B  &  mIoU-N	  &  HM   &  mIoU-B  &  mIoU-N	  &  HM  &  mIoU-B  &  mIoU-N	  &  HM	  \\ \hline
 &  FT                                  &  40.3 & 6.8 & 11.7 & 36.4 & 5.5 & 9.5 & 40.4 & 5.1 & 9.0 & 42.5 & 6.0 & 10.6 & 41.8 & 10.8 & 17.1 \\ \hline
\parbox[t]{2mm}{\multirow{3}{*}{\rotatebox[origin=c]{90}{FSC}}}
 &  WI \cite{qi2018low}                 &  46.5 & 9.3 & 15.4 & 43.2 & 5.8 & 10.3 & 46.1 & 10.0 & 16.4 & 49.1 & 9.5 & 15.9 & 47.5 & 11.7 & 18.8 \\
 &  DWI \cite{gidaris2018dynamic}       &  46.5 & 11.4 & 18.3 & 35.8 & 7.1 & 11.8 & 39.4 & 9.3 & 15.0 & 41.2 & 9.4 & 15.4 & 43.1 & 7.8 & 13.3 \\
 &  RT \cite{tian2020rethinking}        &  43.8 & 10.1 & 16.4 & 38.6 & 5.6 & 9.8 & 44.3 & 11.3 & \underline{18.0 }& 47.0 & 8.7 & 14.6 & 45.2 & 14.7 & 22.2 \\ \hline
\parbox[t]{2mm}{\multirow{2}{*}{\rotatebox[origin=c]{90}{FSS}}}
 &  AMP  \cite{siam2019adaptive}        &  36.0 & 9.2 & 14.6 & 33.2 & 7.9 & 12.8 & 36.7 & 8.9 & 14.3 & 37.9 & 8.7 & 14.2 & 36.4 & 11.2 & 17.2 \\
 &  SPN  \cite{xian2019spnet}           &  41.7 & 12.5 & \underline{19.2} & 38.4 & 8.8 & \underline{14.3} & 41.9 & 10.1 & 16.3 & 44.0 & 13.6 & \textbf{20.8} & 42.5 & 17.3 & \textbf{24.6} \\ \hline
\parbox[t]{2mm}{\multirow{3}{*}{\rotatebox[origin=c]{90}{IL}}}
 &  LwF  \cite{li2017learning}          &  42.7 & 6.5 & 11.3 & 38.1 & 6.3 & 10.9 & 43.3 & 4.9 & 8.8 & 44.6 & 5.6 & 9.9 & 44.7 & 9.4 & 15.5 \\
 &  ILT  \cite{michieli2019incremental} &  47.1 & 10.0 & 16.5 & 46.5 & 7.1 & 12.3 & 48.5 & 8.0 & 13.7 & 47.7 & 13.2 & 20.7 & 45.7 & 11.9 & 18.8 \\
 &  MiB  \cite{cermelli2020modeling}    &  42.7 & 5.2 & 9.3 & 36.9 & 3.4 & 6.3 & 43.6 & 4.0 & 7.3 & 45.6 & 5.9 & 10.4 & 44.8 & 7.5 & 12.8 \\ \hline
 &  \textbf{\ours}                      &  40.1 & 13.1 & \textbf{19.8} & 37.2 & 10.3 & \textbf{16.1} & 39.9 & 12.7 & \textbf{19.2} & 42.4 & 12.7 & \underline{19.6} & 41.0 & 16.8 & \underline{23.8 }\\  

    \end{tabular}}
    \vspace{-4pt} \caption{\SET: COCO-MS 2-shot.} \label{tab:coco-ms-2}
    \vspace{-4pt}
\end{table*}

\begin{table*}[t]
    \centering
    \setlength{\tabcolsep}{3pt} % Default value: 6pt
    \resizebox{\linewidth}{!}
    {\begin{tabular}{ll|ccc||ccc|ccc|ccc|ccc}
     &    &   \multicolumn{3}{c||}{\textbf{Mean}}  &  \multicolumn{3}{c|}{\textbf{20-0}}  &  \multicolumn{3}{c|}{\textbf{20-1}}  &  \multicolumn{3}{c|}{\textbf{20-2}}  &  \multicolumn{3}{c}{\textbf{20-3}} \\ \hline
 &  Method	                          &  mIoU-B  &  mIoU-N	  &  HM	  &  mIoU-B  &  mIoU-N	  &  HM  &  mIoU-B  &  mIoU-N	  &  HM   &  mIoU-B  &  mIoU-N	  &  HM  &  mIoU-B  &  mIoU-N	  &  HM	  \\ \hline
 &  FT                                  &  39.5 & 11.5 & 17.8 & 36.1 & 11.1 & 17.0 & 38.4 & 9.3 & 15.0 & 42.0 & 10.6 & 16.9 & 41.5 & 14.8 & 21.8 \\ \hline
\parbox[t]{2mm}{\multirow{3}{*}{\rotatebox[origin=c]{90}{FSC}}}
 &  WI \cite{qi2018low}                 &  46.3 & 10.3 & 16.8 & 43.4 & 7.3 & 12.4 & 45.7 & 11.1 & 17.8 & 48.7 & 10.5 & 17.2 & 47.4 & 12.3 & 19.5 \\
 &  DWI \cite{gidaris2018dynamic}       &  46.6 & 14.5 & 22.1 & 35.8 & 7.1 & 11.8 & 39.4 & 9.3 & 15.0 & 41.2 & 9.4 & 15.4 & 43.1 & 7.8 & 13.3 \\
 &  RT \cite{tian2020rethinking}        &  44.1 & 16.0 & 23.5 & 39.8 & 11.8 & 18.3 & 44.1 & 16.2 & \textbf{23.7 }& 47.0 & 15.7 & 23.6 & 45.4 & 20.2 & 28.0 \\ \hline
\parbox[t]{2mm}{\multirow{2}{*}{\rotatebox[origin=c]{90}{FSS}}}
 &  AMP  \cite{siam2019adaptive}        &  33.2 & 11.0 & 16.5 & 30.8 & 9.3 & 14.2 & 33.5 & 11.6 & 17.3 & 34.5 & 10.2 & 15.8 & 34.0 & 12.9 & 18.7 \\
 &  SPN  \cite{xian2019spnet}           &  41.4 & 18.2 &\textbf{ 25.3} & 37.9 & 16.8 & \textbf{23.3} & 41.0 & 14.6 & 21.5 & 44.0 & 19.0 & \textbf{26.5 }& 42.8 & 22.4 & \underline{29.4} \\ \hline
\parbox[t]{2mm}{\multirow{3}{*}{\rotatebox[origin=c]{90}{IL}}}
 &  LwF  \cite{li2017learning}          &  42.3 & 12.6 & 19.4 & 38.7 & 12.3 & 18.6 & 41.6 & 10.6 & 16.9 & 44.7 & 11.5 & 18.2 & 44.4 & 16.1 & 23.6 \\
 &  ILT  \cite{michieli2019incremental} &  45.3 & 15.3 & 22.8 & 41.1 & 14.5 & 21.4 & 45.3 & 13.7 & 21.0 & 47.8 & 14.1 & 21.8 & 47.1 & 18.8 & 26.9 \\
 &  MiB  \cite{cermelli2020modeling}    &  43.8 & 11.5 & 18.2 & 38.3 & 10.1 & 16.0 & 44.4 & 9.4 & 15.6 & 46.4 & 11.4 & 18.4 & 46.2 & 14.8 & 22.4 \\ \hline
 &  \textbf{\ours}                      &  41.1 & 18.3 &\textbf{ 25.3} & 38.2 & 16.3 & \underline{22.9} & 39.7 & 15.5 & \underline{22.3} & 43.7 & 18.9 & \underline{26.4} & 42.7 & 22.6 & \textbf{29.5} \\  

    \end{tabular}}
    \vspace{-4pt} \caption{\SET: COCO-MS 5-shot.} \label{tab:coco-ms-5}
    \vspace{-4pt}
\end{table*}

\begin{figure*}[t]
    \centering
    \includegraphics[width=0.98\linewidth]{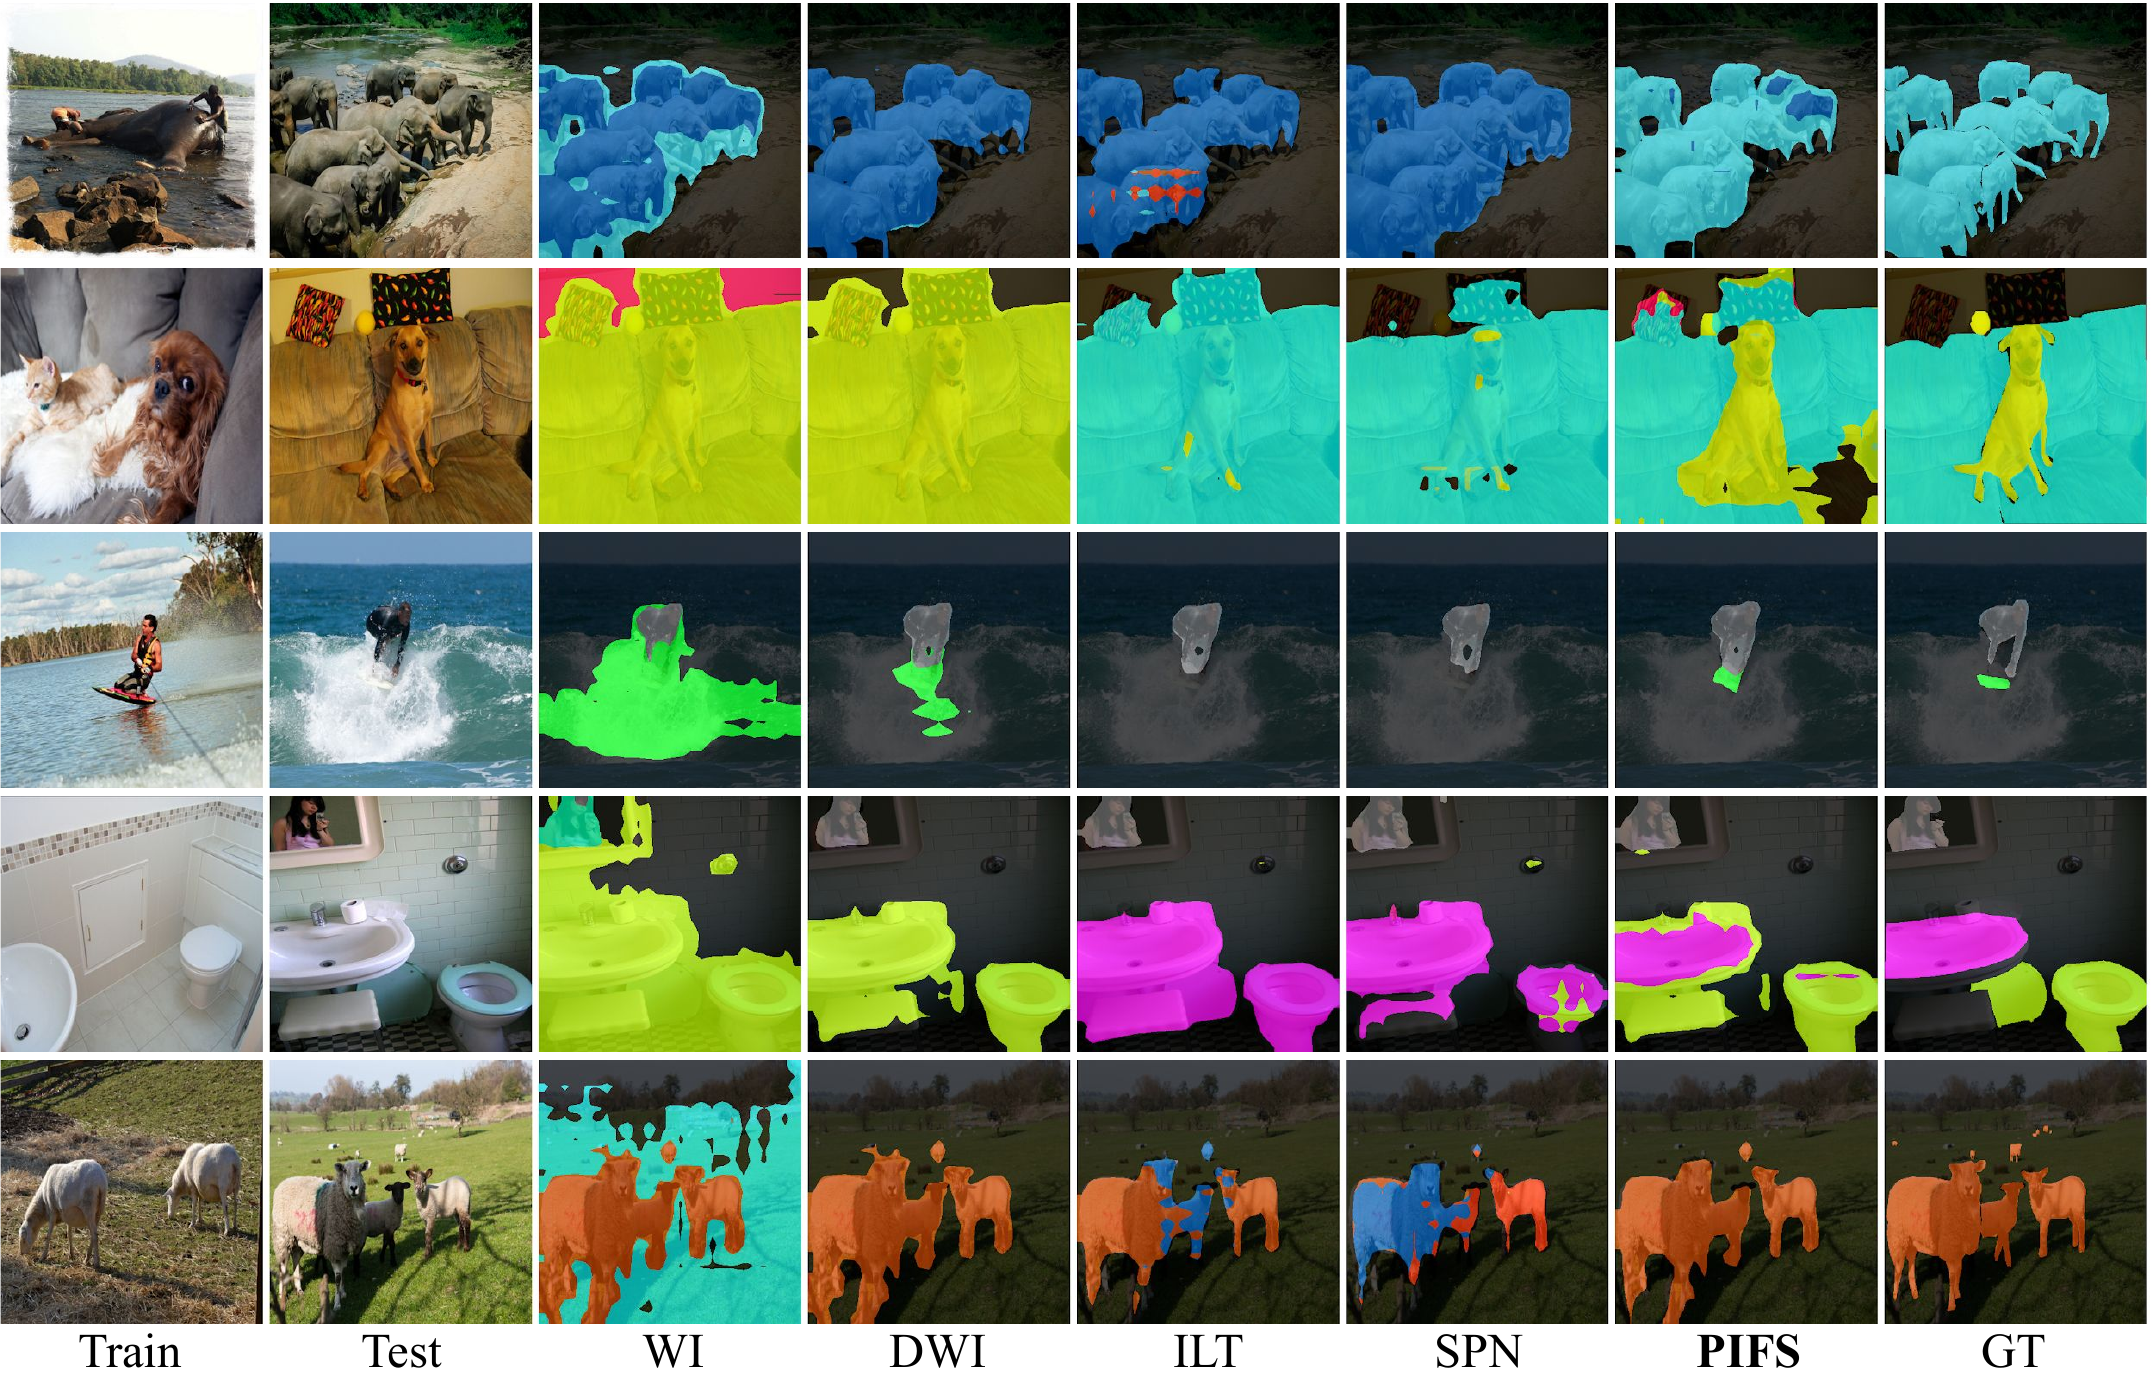}
    \vspace{-8pt}
    \caption{Qualitative results on the COCO-SS 1-shot setting.}
    \label{fig:qualitative-coco}
    \vspace{-4pt}
\end{figure*}

\begin{figure*}[t]
    \centering
    \includegraphics[width=0.98\linewidth]{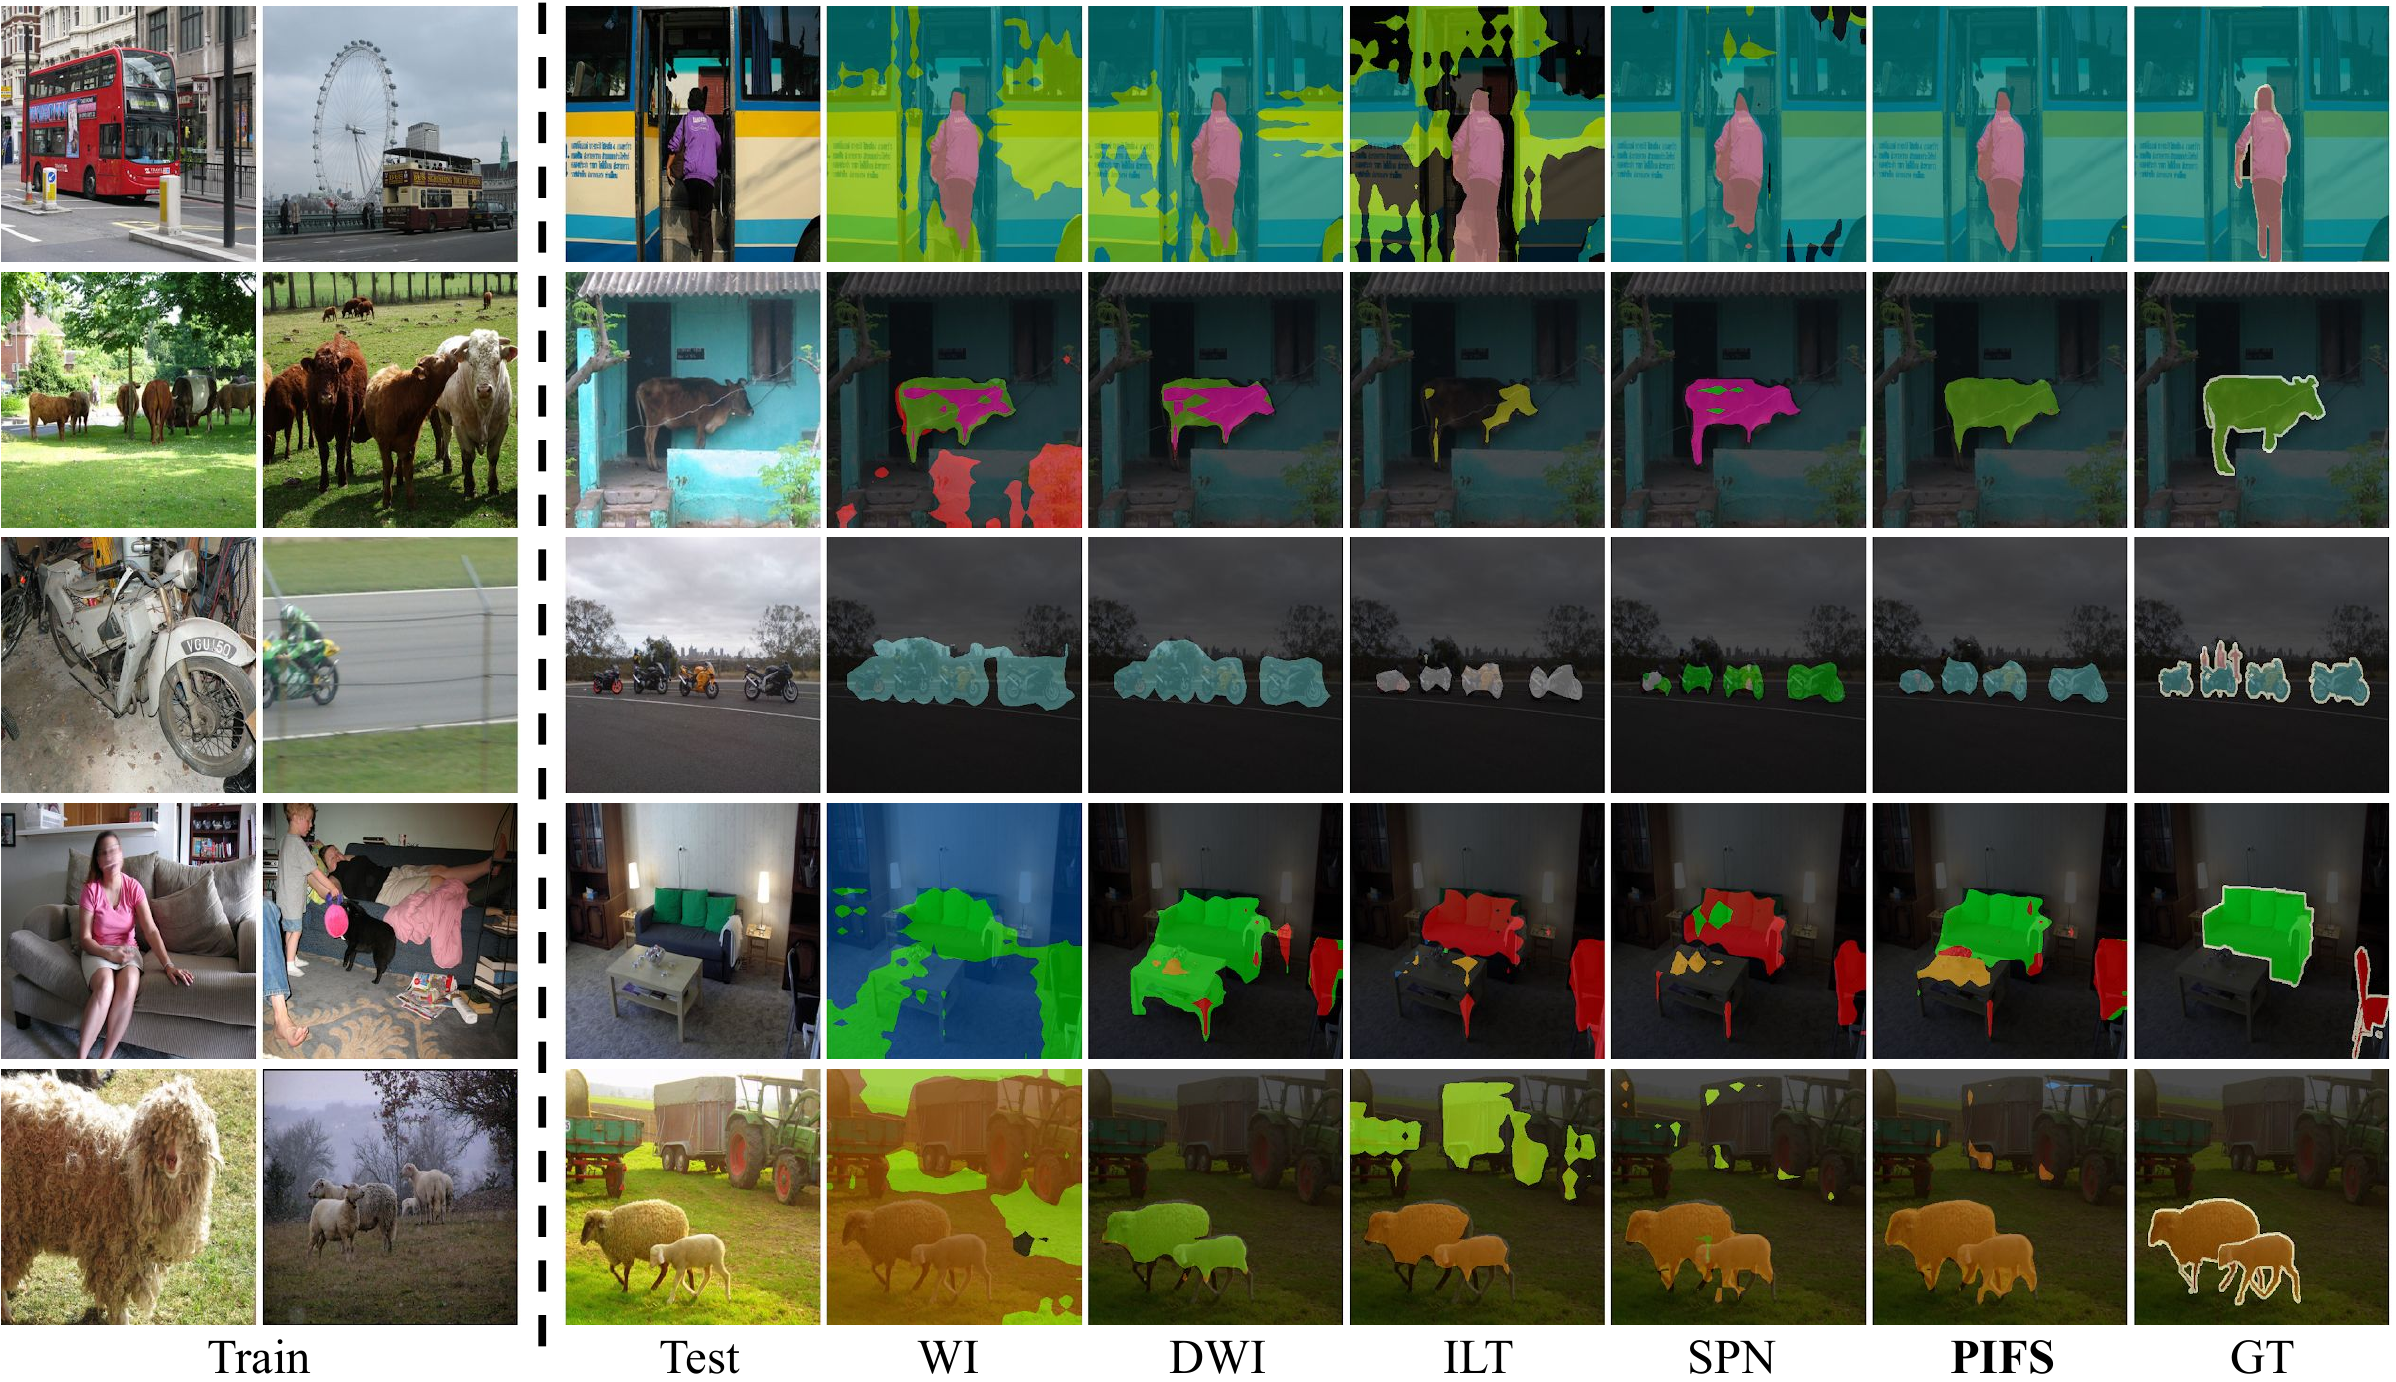}
    \vspace{-8pt}
    \caption{Qualitative results on the VOC-SS 2-shot setting.}
    \label{fig:qualitative-voc2}
    \vspace{-8pt}
\end{figure*}

\begin{figure*}[t]
    \centering
    \includegraphics[width=0.98\linewidth]{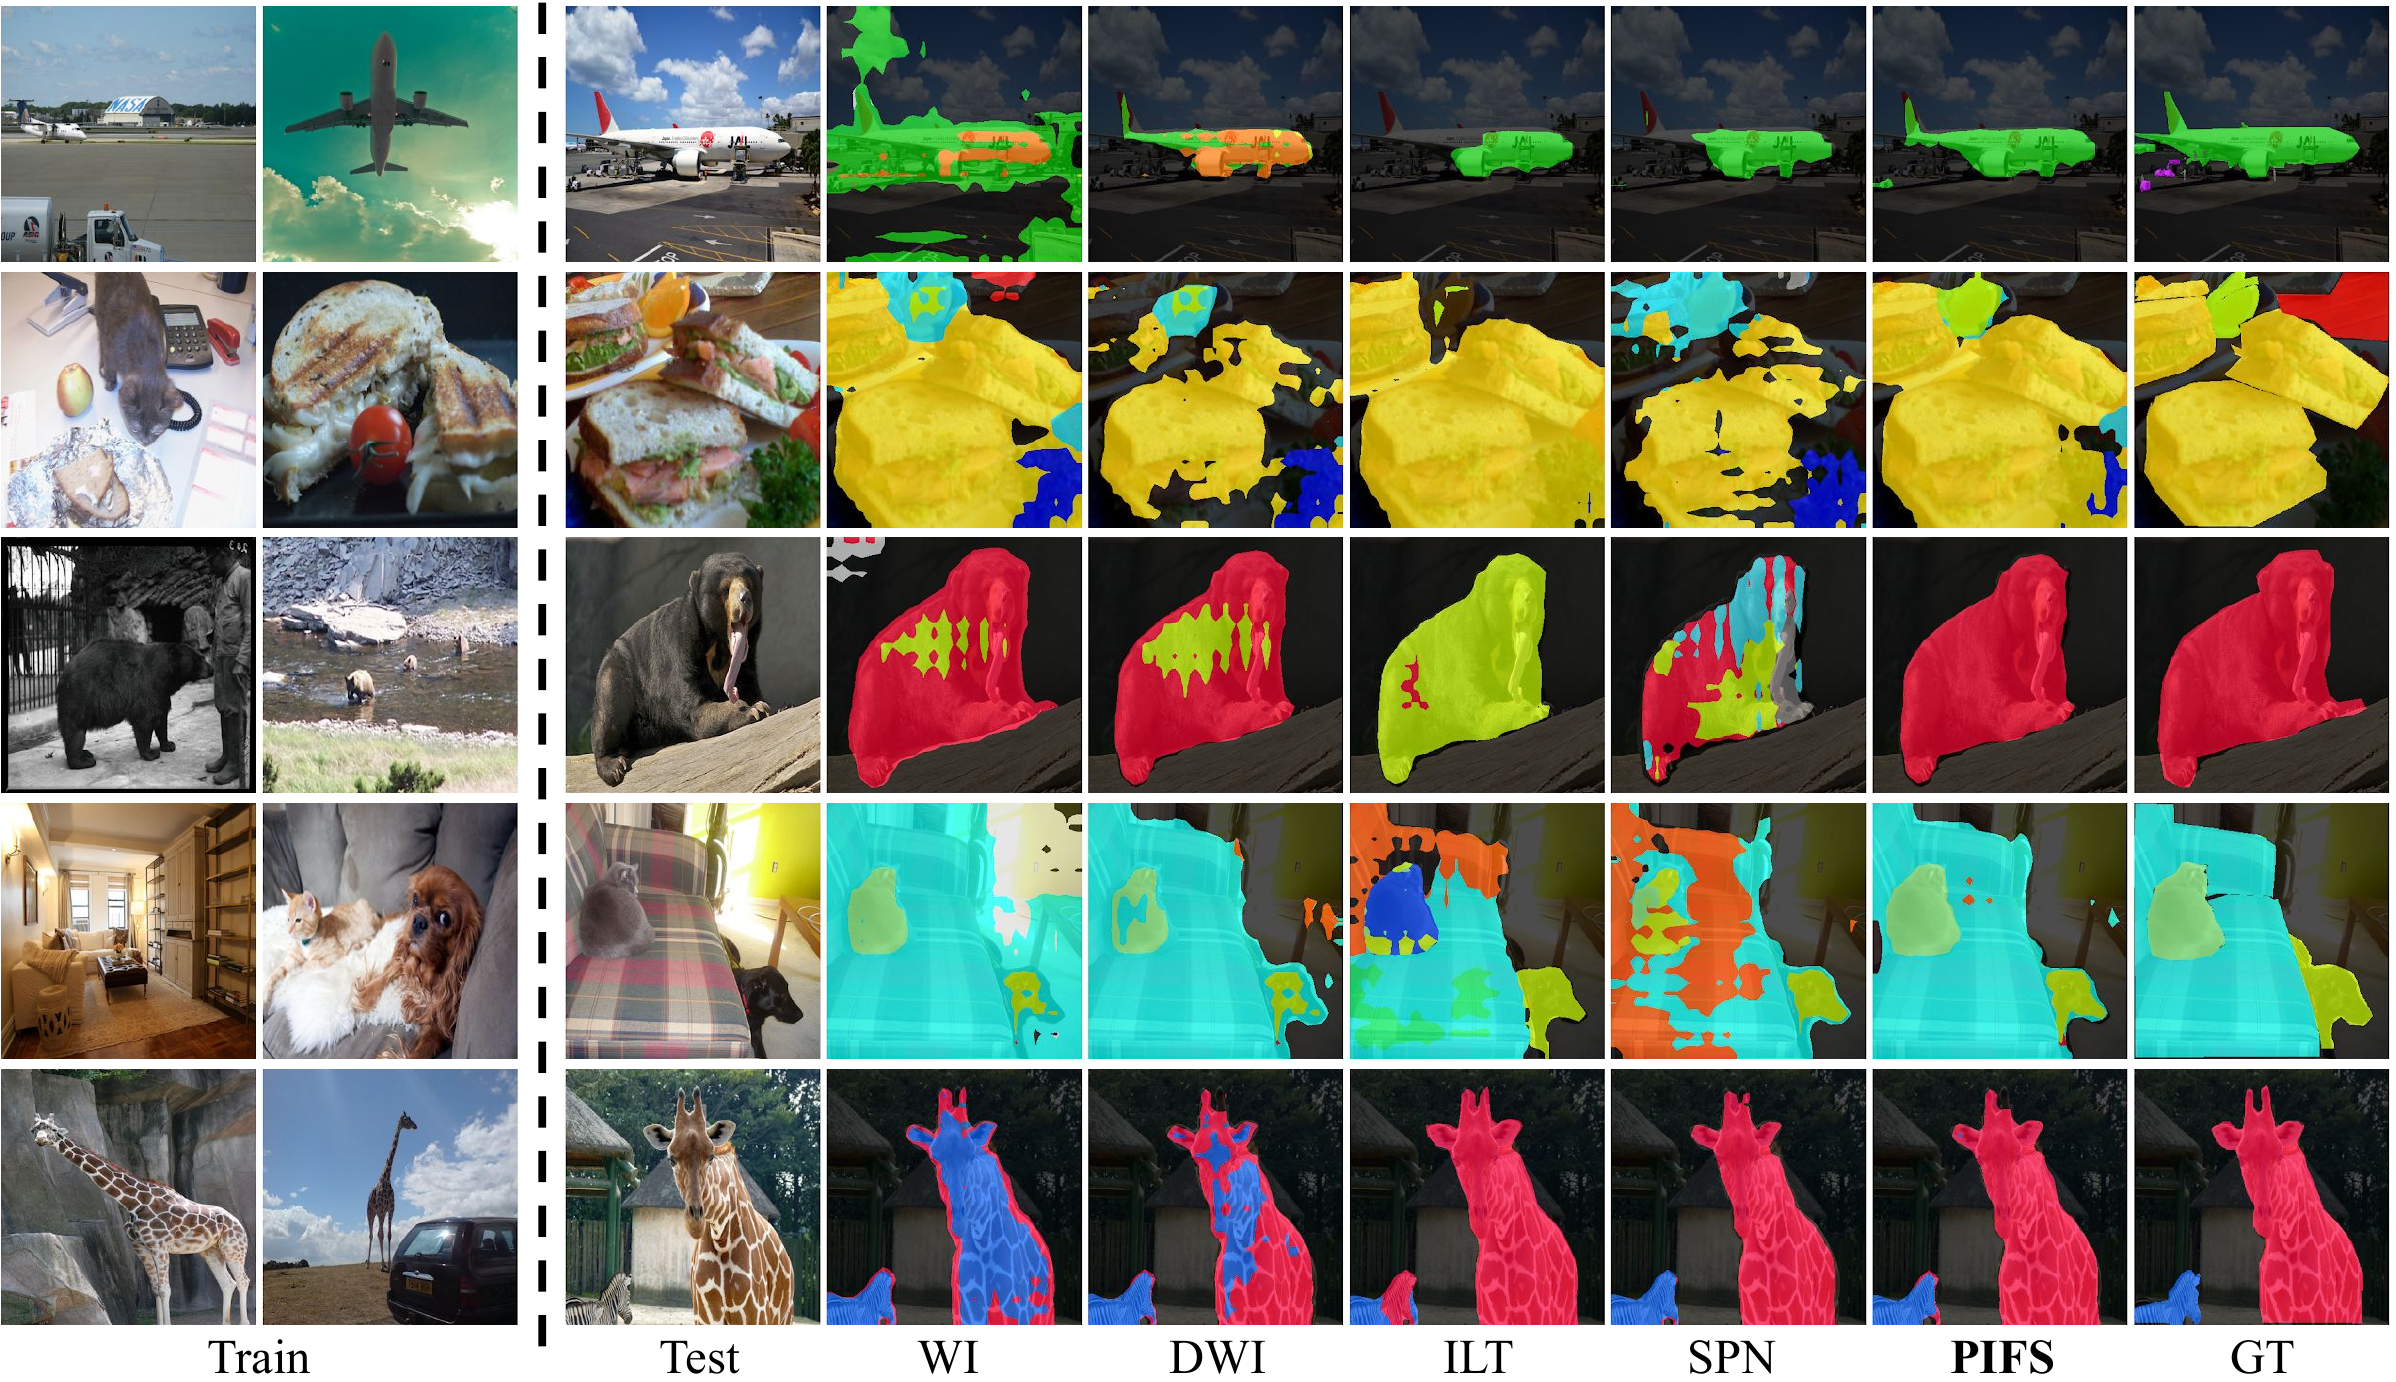}
    \vspace{-8pt}
    \caption{Qualitative results on the COCO-SS 2-shot setting.}
    \label{fig:qualitative-coco2}
    \vspace{-8pt}
\end{figure*}
